# Supplementary material for: What's in a Package? Getting Visibility Into Dependencies Using Security-Sensitive API Calls
Source: arXiv:2408.02846 source file (2026-10-26)
Supplement: Supplementary file 1 [file supplementary.tex]

\documentclass[10pt,conference]{IEEEtran}

\ifCLASSOPTIONcompsoc
  \usepackage[nocompress]{cite}
\else
  \usepackage{cite}
\fi

\usepackage{amsmath,amssymb,amsfonts}
\usepackage{algorithmic}
\usepackage{graphicx}
\usepackage{tabularx}
\usepackage{textcomp}
\usepackage{xcolor}
\usepackage{hhline}
\usepackage{xltabular}

\usepackage{hyperref}
\def\BibTeX{{\rm B\kern-.05em{\sc i\kern-.025em b}\kern-.08em
    T\kern-.1667em\lower.7ex\hbox{E}\kern-.125emX}}

\usepackage[linesnumbered,ruled,vlined]{algorithm2e}
\usepackage{hyperref}
\usepackage{tabulary}

\usepackage{float}

\usepackage{graphics}
\graphicspath{ {./figs/} }

\usepackage{caption}
\usepackage{subcaption}
\usepackage{enumitem}

\usepackage{amsthm}

\usepackage{booktabs}

\usepackage{makecell}
\usepackage{multirow}

\usepackage{mathtools,tikz,caption}
\captionsetup{labelfont=sc,labelsep=period}
\DeclareRobustCommand\sampleline[1]{%
    \tikz\draw[#1] (0,0) (0,\the\dimexpr\fontdimen22\textfont2\relax)
    -- (2em,\the\dimexpr\fontdimen22\textfont2\relax);%
}

\usepackage[most]{tcolorbox}

\usepackage{soul}

\definecolor{color-up-to-date}{HTML}{8CC5E3}
\definecolor{color-tood}{HTML}{2066A8}
\definecolor{color-pfet-tood}{HTML}{F72B8F}

\usepackage{lipsum}                     %
\usepackage{xargs}                      %
\usepackage[colorinlistoftodos,prependcaption,textsize=scriptsize]{todonotes}
\newcommandx{\unsure}[2][1=]{\todo[linecolor=red,backgroundcolor=red!25,bordercolor=red,#1]{#2}}
\newcommandx{\change}[2][1=]{\todo[linecolor=blue,backgroundcolor=blue!25,bordercolor=blue,#1]{#2}}
\newcommandx{\info}[2][1=]{\todo[linecolor=OliveGreen,backgroundcolor=OliveGreen!25,bordercolor=OliveGreen,#1]{#2}}
\newcommandx{\improvement}[2][1=]{\todo[linecolor=Plum,backgroundcolor=Plum!25,bordercolor=Plum,#1]{#2}}
\newcommandx{\thiswillnotshow}[2][1=]{\todo[disable,#1]{#2}}

\long\def\longcaption#1#2{\centering\begin{minipage}{#1}\vspace{-0.7\baselineskip}\footnotesize\noindent\emph{#2}\end{minipage}}

\SetCommentSty{mycommfont}

\newcommand{\sensapi}{security-sensitive API\xspace}

\newcommand{\Sensapis}{Security-sensitive APIs\xspace} %
\newcommand{\SenSapi}{Security-Sensitive API\xspace}

\SetKwInput{KwInput}{Input}                %
\SetKwInput{KwOutput}{Output}              %
\SetKwInput{KwNotation}{Notation}

\newcounter{rqcounter}
\setcounter{rqcounter}{0}

\newcommand\pkgname[1]{\textsf{\small #1}}
\newcommand\api[1]{\textit{#1}}
\newcommand\apicat[1]{\textsc{\small #1}}

\begin{document}

\title{Less Is More: A Mixed-Methods Study on \SenSapi Calls in Java for Better Dependency Selection \\ {\large SUPPLEMENTARY MATERIAL} }
\maketitle

\onecolumn

\section{\Sensapis in Package Groups}

\noindent \textbf{Dependency Injection.}
Dependency injection is a software design pattern that allows the removal of hard-coded dependencies and makes it possible to change them, whether at runtime or compile time.
\pkgname{Spring-beans} and \pkgname{spring-context} used 368 and 235 \apicat{reflection} APIs, respectively, which are the highest and second-highest by any dependency injector framework.
High use of \apicat{reflection} APIs indicates that \pkgname{spring-beans} and \pkgname{spring-context} change the dependencies at runtime.
\pkgname{Guice} and \pkgname{jakarta.enterprise.cdi-api} used 66 and 9 \apicat{reflection} API calls, respectively, to achieve similar functionality as \pkgname{spring-beans} and \pkgname{spring-context}.
On the other hand, \pkgname{dagger} used 0 API calls, which indicates that it does not even use reflection to change the dependencies at runtime.

\noindent \textbf{HTTP Client.}
HTTP client packages provide the implementation of HTTP methods (e.g., GET and POST).
All the HTTP client packages in our set use minimal calls to the \apicat{network} category,
indicating an optimized implementation with good software engineering practices,
i.e. on average, they call one API in \apicat{network/connection} and three in \apicat{network/socket}. 
All the packages in this group use \apicat{process/reflection} and \apicat{process/codec\_crypto} APIs.
The use of \apicat{process/codec\_crypto} APIs indicates that encoding/decoding and encryption/decryption are necessary for network communications in these packages.
Interestingly, \pkgname{retrofit} uses \pkgname{okhttp} as a dependency, but it uses fewer calls in each API category (except \apicat{process/reflection}) compared to \pkgname{okhttp}.
The reasoning is our call-graph generator stitches the \textit{reachable} calls from the entry points of the package to dependency, and so \pkgname{retrofit} achieves the same functionality with fewer calls than \pkgname{okhttp} by making minimal calls only to \pkgname{okhttp}.

\noindent \textbf{I/O Utilities.}
I/O utility packages provide the implementation of I/O operations such as reading, writing, and modifying files complementing \api{java.io} and \api{java.nio} packages.
All I/O utilities use every \apicat{filesystem} category 
except \apicat{read\_network\_env} with \apicat{filesystem/miscellaneous} as the most used API category.
The only package that uses \apicat{read\_network\_env} is \pkgname{jetty-io}.
Moreover, all the packages use the \apicat{process/reflection} and \apicat{network/connection} categories.
Also in the \apicat{network} category, \pkgname{jetty-io} is the only package that calls the \apicat{network/socket} and \apicat{naming\_directory} APIs, once each.

\noindent \textbf{JDBC Drivers.}
JDBC (Java Database Connectivity) driver packages allow Java applications to interact with databases.
\apicat{Process/reflection}, \apicat{filesystem/read\_env}, and \apicat{process/codec\_crypto} APIs are the top three used API categories by JDBC drivers.
\pkgname{Sqlite-jdbc} is the package with the lowest API calls in this category.
Interestingly, \pkgname{sqlite-jdbc} does not use any \apicat{filesystem/input} or \apicat{output} APIs.
Other than that, \apicat{filesystem/read\_env} APIs are used by all JDBC drivers to read environment variables and configuration files.

\noindent \textbf{JSON Libraries.}
JSON libraries provide the implementation of JSON parsing and serialization to Java objects, and vice versa.
\pkgname{Fastjson2} extensively uses \apicat{process/reflection} APIs compared to \pkgname{gson} and \pkgname{jackson-core}.
\pkgname{Fastjson2} has more functionality than the others, and this is reflected in its API usage, i.e., parsing objects from URLs (\apicat{network/connection} APIs) and Base64 encoded strings (\apicat{process/codec\_crypto} APIs).

\noindent \textbf{Logging.}
Logging libraries provide the implementation of logging functionality in Java applications.
\pkgname{Log4j-core} and \pkgname{logback-classic} use five out of six \apicat{filesystem} categories
and \apicat{process/reflection} is the most used API category by these two libraries.

\noindent \textbf{Web Frameworks.}
Web frameworks support the development of web applications, including web services, web resources, and web APIs.
All the web frameworks extensively use \apicat{process/reflection} to load classes and methods dynamically.
For example, \pkgname{spring-web} uses \apicat{reflection} APIs to load the classes written by the developer and to create objects of those classes, manipulate them, and inject them into other classes.
The \apicat{filesystem} category calls do not fluctuate much across the web frameworks.
The only exception is \pkgname{tapestry-core}, which has 157 indirect calls to \apicat{filesystem/output}.
The only package in this group that uses \apicat{process/operating\_system} APIs (indirectly) is \pkgname{struts2-core}.

\noindent \textbf{XML Parsers.}
XML parsers provide utilities to parse, transform, serialize, and query XML documents.
All XML processors only use \apicat{connection} from the \apicat{network} category and \apicat{reflection} from the \apicat{process} category.
\apicat{Filesystem} APIs are uniformly used by the XML processors.
\pkgname{Dom4j} and \pkgname{xstream} both use \apicat{filesystem/input} and \apicat{miscellaneous} APIs whereas \pkgname{jakarta.xml.bind-api} and \pkgname{jaxb-api} do not.
The most used API category by XML parsers is the \apicat{process/reflection} category and \pkgname{xstream} makes the highest number of (direct + indirect) calls to this category (it used \pkgname{jaxb-api} as a dependency).

\noindent \section{Full API list}

\begin{xltabular}{\linewidth}{lll}
  \caption{Security-sensitive Java API List}\\
  \toprule \textbf{Category} & \textbf{Subcategory} & \textbf{APIs}\\ \midrule
  \endfirsthead
  \endhead
  \multicolumn{3}{r}{{Continued on next page}} \\ 
  \endfoot
  \multicolumn{3}{r}{{End}} \\
  \endlastfoot
  \label{tab:full_list}
        & & java.io.FileInputStream() \\
        & & java.io.FileReader() \\
        & & java.nio.channels.FileChannel.read() \\
        & & java.nio.file.Files.lines() \\
        & & java.nio.file.Files.newBufferedReader() \\
        & & java.nio.file.Files.newInputStream() \\
        & & java.nio.file.Files.readAllBytes() \\
        & & java.nio.file.Files.readAllLines() \\
        & & java.nio.file.Files.readString() \\
        & & java.nio.file.Files.readSymbolicLink() \\
        & & java.util.Scanner() \\
        & & javax.xml.parsers.DocumentBuilder.parse() \\
        & \multirow{-13}{*}{\apicat{Input}} & javax.xml.parsers.SAXParser.parse()\\
        \hhline{~--}
        & & java.io.File() \\
        & & java.io.File.exists()\\
        & & java.io.File.getAbsolutePath() \\
        & & java.io.File.getCanonicalFile() \\
        & & java.io.File.getPath() \\
        & & java.io.File.toPath() \\
        & & java.io.RandomAccessFile() \\
        & & java.nio.channels.FileChannel() \\
        & & java.nio.file.Paths.get() \\
        & & java.security.BasicPermission() \\
        & \multirow{-11}{*}{\apicat{Miscellaneous}} & java.security.ProtectionDomain() \\
        \hhline{~--}
        & & java.nio.file.Files.copy() \\
        & & java.nio.file.Files.delete() \\
        & & java.nio.file.Files.deleteIfExists() \\
        & & java.nio.file.Files.move() \\
        \apicat{Filesystem} & \multirow{-5}{*}{\apicat{Modification}} & java.nio.file.Files.newByteChannel() \\ \hhline{~--}
        & & java.io.File.createTempFile() \\
        & & java.io.File.mkdir() \\
        & & java.io.FileOutputStream() \\
        & & java.io.FileWriter() \\
        & & java.nio.file.Files.createFile() \\
        & & java.nio.file.Files.createLink() \\
        & & java.nio.file.Files.createSymbolicLink() \\
        & & java.nio.file.Files.createTempFile() \\
        & & java.nio.file.Files.newBufferedWriter() \\
        & & java.nio.file.Files.newOutputStream() \\
        & & java.nio.file.Files.setLastModifiedTime() \\
        & & java.nio.file.Files.setOwner() \\
        & & java.nio.file.Files.setPosixFilePermissions() \\
        & & java.nio.file.Files.write() \\
         & & java.nio.file.Files.writeString() \\
        & & java.util.logging.Logger.info()\\
        & \multirow{-17}{*}{\apicat{Output}}  & java.util.logging.Logger.log() \\
        \hhline{~--}
        & & java.lang.ProcessBuilder.environment() \\
        & & java.lang.System.getenv() \\
        & & java.lang.System.getProperties() \\
        & & java.lang.System.getProperty() \\
        & & java.lang.System.getSecurityManager() \\
        & & java.sql.Connection.getMetaData() \\
        & & java.util.Properties.getProperty() \\
        & & java.util.Properties.setProperty() \\
        & \multirow{-10}{*}{\apicat{Read\_env}} & java.util.Properties() \\
        \hhline{~--}
        & & java.net.InetAddress.getAllByName() \\
        & & java.net.InetAddress.getHostAdress() \\
        & & java.net.InetAddress.getHostName() \\
        & & java.net.InetAddress.getLocalHost() \\
        & & java.net.InetAddress.getLoopbackAddress() \\
        & & java.net.InetAddress.isReachable() \\
        & & java.net.InetSocketAddress() \\
        & & java.net.InetSocketAddress.getHostName() \\
        & & java.net.InetSocketAddress.getPort() \\
        & & java.net.NetworkInterface.getInetAddresses() \\
        & & java.net.Socket.getInetAdress() \\
        & & java.net.URI() \\
        & & java.net.URI.getAuthority()  \\
        & & java.net.URI.getHost() \\
        & & java.net.URI.getPort()  \\
        & & java.net.URI.getRawSchemeSpecificPart() \\
        & & javax.servlet.http.HttpServletRequest.getContextPath() \\
        & & javax.servlet.http.HttpServletRequest.getLocalAddr() \\
        & & javax.servlet.http.HttpServletRequest.getLocalName() \\
        & & javax.servlet.http.HttpServletRequest.getLocalPort() \\
        & & javax.servlet.http.HttpServletRequest.getRemoteAddr() \\
        & & javax.servlet.http.HttpServletRequest.getRemotePort() \\
        & & javax.servlet.http.HttpServletRequest.getQueryString() \\
        & & javax.servlet.http.HttpServletRequest.getRequestURI() \\
        & & javax.servlet.http.HttpServletRequest.getServletPath() \\
        & \multirow{-27}{*}{\apicat{Read\_network\_env}} &  javax.servlet.http.HttpServletResponse.setStatus() \\
        \midrule \midrule
        & & jakarta.servlet.ServletContext.getRequestDispatcher() \\
        & & java.net.HttpsURLConnection() \\
        & & java.net.HttpsURLConnection.connect() \\
        & & java.net.HttpURLConnection() \\
        & & java.net.HttpURLConnection.connect() \\
        & & java.net.HttpURLConnection.getInputStream() \\
        & & java.net.HttpURLConnection.getOutputStream() \\
        & & java.net.JarURLConnection() \\
        & & java.net.JarURLConnection.connect() \\
        & & java.net.URL() \\
        & & java.net.URL.openConnection() \\
        & & java.net.URL.openStream() \\
        & & java.sql.DriverManager.getConnection()\\
        & & java.sql.Statement.executeQuery()\\
        & & javax.servlet.http.HttpServletRequest.getRequestDispatcher() \\
        & \multirow{-16}{*}{\apicat{Connection}} & javax.sql.DataSource.getConnection() \\ \hhline{~--}
        & & jakarta.servlet.http.HttpServletRequest.getParameter()\\
        & & jakarta.servlet.http.HttpServletRequest.getRequestDispatcher() \\
        \apicat{Network} & & jakarta.servlet.http.HttpServletRequest.setAttribute() \\
        & & jakarta.servlet.http.HttpServletResponse.getWriter()\\
        & & jakarta.servlet.http.HttpServletResponse.setStatus() \\
        & & java.net.http.HttpClient() \\
        & & java.net.http.HttpClient.Builder.build() \\
        & & java.net.http.HttpClient.newBuilder() \\
        & & java.net.http.HttpClient.newHttpClient() \\
        & & java.net.http.HttpClient.send() \\
        & & java.net.http.HttpClient.sendAsync() \\
        & & javax.net.ssl.HttpsURLConnection.setHostnameVerifier()\\
        & & javax.security.auth.login.LoginContext.login()\\
        & & javax.servlet.http.Cookie() \\
        & & javax.servlet.http.HttpServlet() \\
        & & javax.servlet.http.HttpServletResponse.addHeader \\ 
        & & javax.servlet.http.HttpServletResponse.getWriter()\\
        & & javax.servlet.http.HttpServletResponse.sendRedirect()\\
        & & javax.servlet.http.HttpServletRequest.getParameter()\\
        & & javax.servlet.http.HttpServletRequestWrapper() \\
        & & javax.servlet.http.HttpSession.getAttribute()\\
        & \multirow{-21}{*}{\apicat{Http}} & javax.servlet.http.HttpSession.setAttribute()\\
        \hhline{~--}
        & & javax.naming.Context() \\
        & & javax.naming.Context.bind() \\
        & & javax.naming.Context.list() \\
        & & javax.naming.Context.listBindings() \\
        & & javax.naming.Context.lookup() \\
        & & javax.naming.Context.lookupLink() \\
        & & javax.naming.Context.rebind() \\
        & & javax.naming.Context.rename() \\
        & & javax.naming.Context.unbind() \\
        & & javax.naming.directory.DirContext() \\
        & & javax.naming.directory.InitialDirContext() \\
        & & javax.naming.InitialContext() \\
        & \multirow{-13}{*}{\apicat{Naming\_directory}} & javax.naming.InitialContext.lookup() \\\hhline{~--}
        & & java.net.DatagramSocket()\\
        & & java.net.DatagramSocket.connect()\\
        & & java.net.http.HttpClient.newWebSocketBuilder()\\
        & & java.net.http.WebSocket.Builder.buildAsync()\\
        & & java.net.http.WebSocket.sendBinary()\\
        & & java.net.http.WebSocket.sendPing()\\
        & & java.net.http.WebSocket.sendPong()\\
        & & java.net.http.WebSocket.sendText()\\
        & & java.net.ServerSocket()\\
        & & java.net.ServerSocket.accept()\\
        & & java.net.Socket()\\
        & & java.net.Socket.connect()\\\
        & & java.net.Socket.getInputStream()\\
        & & java.nio.channels.ServerSocketChannel()\\
        & & java.nio.channels.ServerSocketChannel.socket()\\
        & & java.nio.channels.SocketChannel()\\
        & & java.rmi.server.RMISocketFactory()\\
        & & java.rmi.server.RMISocketFactory.createServerSocket()\\
        & & java.rmi.server.RMISocketFactory.createSocket()\\
        & \multirow{-22}{*}{\apicat{Socket}} & javax.websocket.WebSocketContainer()\\
         \midrule \midrule
         & & java.net.URLDecoder.decode() \\
        & & java.net.URLEncoder.encode() \\
        & & java.nio.charset.CharsetDecoder.charset() \\
        & & java.nio.charset.CharsetEncoder.charset() \\
        & & java.security.MessageDigest.getInstance() \\
        & & java.security.MessageDigest() \\
        & & java.util.Base64.Decoder.decode() \\
        & & java.util.Base64.Decoder.wrap() \\
        & & java.util.Base64.Encoder.encode() \\
        & & java.util.Base64.Encoder.encodeToString() \\
        & & java.util.Base64.Encoder.wrap() \\
        & & java.util.Base64.getDecoder() \\
        & & java.util.Base64.getEncoder() \\
        & & javax.crypto.Cipher.doFinal() \\
        & & javax.crypto.Cipher.getInstance() \\
        & & javax.crypto.Cipher.init() \\
        & & javax.crypto.Cipher.update() \\
        & & javax.crypto.Cipher.updateAAD() \\
        & & javax.crypto.Cipher.wrap() \\
        & & javax.websocket.Decoder.Binary.decode() \\
        & \multirow{-21}{*}{\apicat{Codec\_crypto}} & javax.websocket.Decoder.Text.decode() \\\hhline{~--}  
        & & java.lang.Runtime.load()\\
        & & java.lang.Runtime.loadLibrary()\\
        & & java.lang.System.load()\\
        & \multirow{-4}{*}{\apicat{Dependency}} & java.lang.System.loadLibrary()\\\hhline{~--} 
        & & java.awt.Desktop.open()\\
        & & java.lang.ProcessBuilder.start()\\
        & & java.lang.ProcessBuilder()\\
        \apicat{Process} & \multirow{-4}{*}{\apicat{Operating\_system}}& java.lang.Runtime.exec()\\\hhline{~--} 
         & & java.beans.Introspector.getBeanInfo() \\
        & & java.beans.PropertyDescriptor() \\
        & & java.beans.PropertyDescriptor.getWriteMethod() \\
        & & java.io.ObjectInputStream.readObject() \\
        & & java.lang.Class.forName() \\
        & & java.lang.Class.getConstructor() \\
        & & java.lang.Class.getConstructors() \\
        & & java.lang.Class.getDeclaredConstructor() \\
        & & java.lang.Class.getDeclaredConstructors() \\
        & & java.lang.Class.getDeclaredMethod() \\
        & & java.lang.Class.getDeclaredMethods() \\
        & & java.lang.Class.getMethod() \\
        & & java.lang.Class.getMethods() \\
        & & java.lang.Class.getSuperclass() \\
        & \apicat{Reflection} & java.lang.Class.newInstance() \\
        & & java.lang.ClassLoader() \\
        & & java.lang.ClassLoader.defineClass() \\
        & & java.lang.reflect.AccessibleObject.setAccessible() \\
        & & java.lang.reflect.Constructor.newInstance() \\
        & & java.lang.reflect.Method.getDeclaringClass() \\
        & & java.lang.reflect.Method.invoke() \\
        & & java.net.URLClassLoader() \\
        & & java.net.URLClassLoader.newInstance() \\
        & & java.rmi.server.RMIClassLoader.getClassLoader() \\
        & & java.rmi.server.RMIClassLoader.loadClass() \\
        & & java.util.ServiceLoader.load() \\
        & & java.util.ServiceLoader.loadInstalled() \\\hhline{~--} 
        & & javax.script.ScriptEngine.eval() \\
        & & javax.script.ScriptEngineFactory.getScriptEngine() \\
        & & javax.script.ScriptEngineManager() \\
        & & javax.script.ScriptEngineManager.getEngineByExtension() \\
        & & javax.script.ScriptEngineManager.getEngineByMimeType() \\
        & & javax.script.ScriptEngineManager.getEngineByName() \\
        & & javax.script.ScriptEngineManager.getEngineFactories() \\
        & & jdk.jshell.JShell.Builder.build() \\
        & & jdk.jshell.JShell.builder() \\
        & & jdk.jshell.JShell.create() \\
        & & jdk.jshell.JShell.eval() \\
        & \multirow{-13}{*}{\apicat{Scripting}} & jdk.nashorn.api.scripting.NashornScriptEngine.eval() \\
         \bottomrule
\end{xltabular}

\section{Analysis on CVEs and Vulnerable Functions}
\begin{table}[htbp]
\setlength{\tabcolsep}{3pt}
    \centering
    \caption{Security-sensitive API Calls in Vulnerable Functions}
    \longcaption{0.6\linewidth}{
    The Pkg (avg) row shows the data statistic from the package granularity if we took the average number of API calls for each package. The Pkg (max) row shows the data statistic from the package granularity if we took the maximum API calls for each package. 
    \textbf{Observation:} Half of the package versions have at least 1 call to a \sensapi. }
    
    \begin{tabular}{l|r|rrrrr|rr}
        \toprule
        Unit & \# & Min & Q25\% & Med & Q75\% & Max & Mean & Std.Dev \\
        \midrule
        Pkg vers & 2807 & 0 & 0 & 1 & 7 & 206 & 6.98 & 18.81 \\ 
        Pkg (avg) & 44 & 0 & 0 & 0.92 & 4.94 & 84.84 & 5.01 & 13.16 \\
        Pkg (max) & 44 & 0 & 0 & 2 & 11 & 206 & 9.84 & 30.75 \\
        \bottomrule
    \end{tabular}
    \label{tab:stat_vuln_func}
\end{table}

\begin{table}[htbp]
    \centering
    \caption{CVE Distribution in the Chosen Packages}
    \longcaption{\columnwidth}{}
    \begin{tabular}{llrr}
    \toprule
        OWASP ID & Description & \#CWE & \#CVE \\
        \midrule
        A01 & Broken Access Control & 14 & 41 \\
        A02 & Cryptographic Failures & 3 & 6 \\
        A03 & Injection & 11 & 40 \\
        A04 & Insecure Design & 5 & 15 \\
        A05 & Security Misconfiguration & 2 & 5 \\
        A06 & Vulnerable and Outdated Components & 0 & 0 \\
        A07 & Identification and Authentication Failures & 2 & 3 \\
        A08 & Software and Data Integrity Failures & 4 & 79 \\
        A09 & Security Logging and Monitoring Failures & 1 & 1 \\
        A10 & Server-Side Request Forgery (SSRF) & 1 & 1 \\ \midrule
        Other & Outside the OWASP categorization & 30 & 79 \\
        NoInfo & Insufficient Information &  & 26 \\
        None & No CWE Assigned &  & 3 \\
        \midrule
        \multicolumn{2}{l}{Total} & 73 & 299 \\
        \bottomrule
    \end{tabular}
    \label{tab:owasp}
\end{table}
\newpage
\section{Survey}

\begin{table*}[htbp]
    \setlength{\tabcolsep}{3pt}
    \centering
    \caption{Developer Survey Questions}
    \begin{tabularx}{\textwidth}{p{0.28\columnwidth}p{0.52\columnwidth}p{0.16\columnwidth}}
        \toprule
         Measured Variable & Question & Answer form  \\
         \midrule
        Expectation before information & When you adopt library X in your project which kind of \sensapi categories would you expect to be called from library X? & (A) Checkbox category \\
        Perception & If you had known this \sensapi information before choosing the dependency, how would it affect your decision? & (B) Multiple choice \\
        Perception reasoning & Please elaborate on your choice from the previous question (e.g., why). & (C) Text \\
        API sensitivity & In your opinion, which of the following API categories should be considered sensitive for any package? & (A) Checkbox category \\
        API sensitivity details & Based on your answer to the previous question, what is the degree of sensitivity for your selected API categories? & (D) 10-points Likert scale \\ 
        \midrule
        PILOT ONLY & \\
        \midrule
        Survey clarity & Please rate the clarity of this survey & (E) 5-points Likert scale\\
        Survey visualization comprehensibility & Please rate the comprehensibility/understandability of the visualizations & (E) 5-points Likert scale\\
        \bottomrule
    \end{tabularx}
    \label{tab:survey}
    \begin{minipage}{0.9\textwidth}%
    \vspace{0.5\baselineskip}
    \begin{description}
        \item[(A)] Checkbox with 15 \sensapi categories.
        \item[(B)] Multiple choice
        \item[(C)] Text: open-ended text field
        \begin{itemize}[noitemsep,topsep=0pt,leftmargin=5pt]
            \item keep using chosen dependency 
            \item keep using chosen dependency but will consider for the future
            \item select dependency with the lowest usage
            \item select dependency based on call in a category
            \item other (please specify).
        \end{itemize}
        \item[(D)] 10-point Likert scale: 1 is the least sensitive and 10 is the most sensitive.
        \item[(E)] 5-point Likert scale: very negative, somewhat negative, neither-negative-nor-positive, somewhat positive, very positive
    \end{description}
    \end{minipage}
\end{table*}

\begin{figure}[htbp]
    \centering
    \includegraphics[width=0.7\columnwidth]{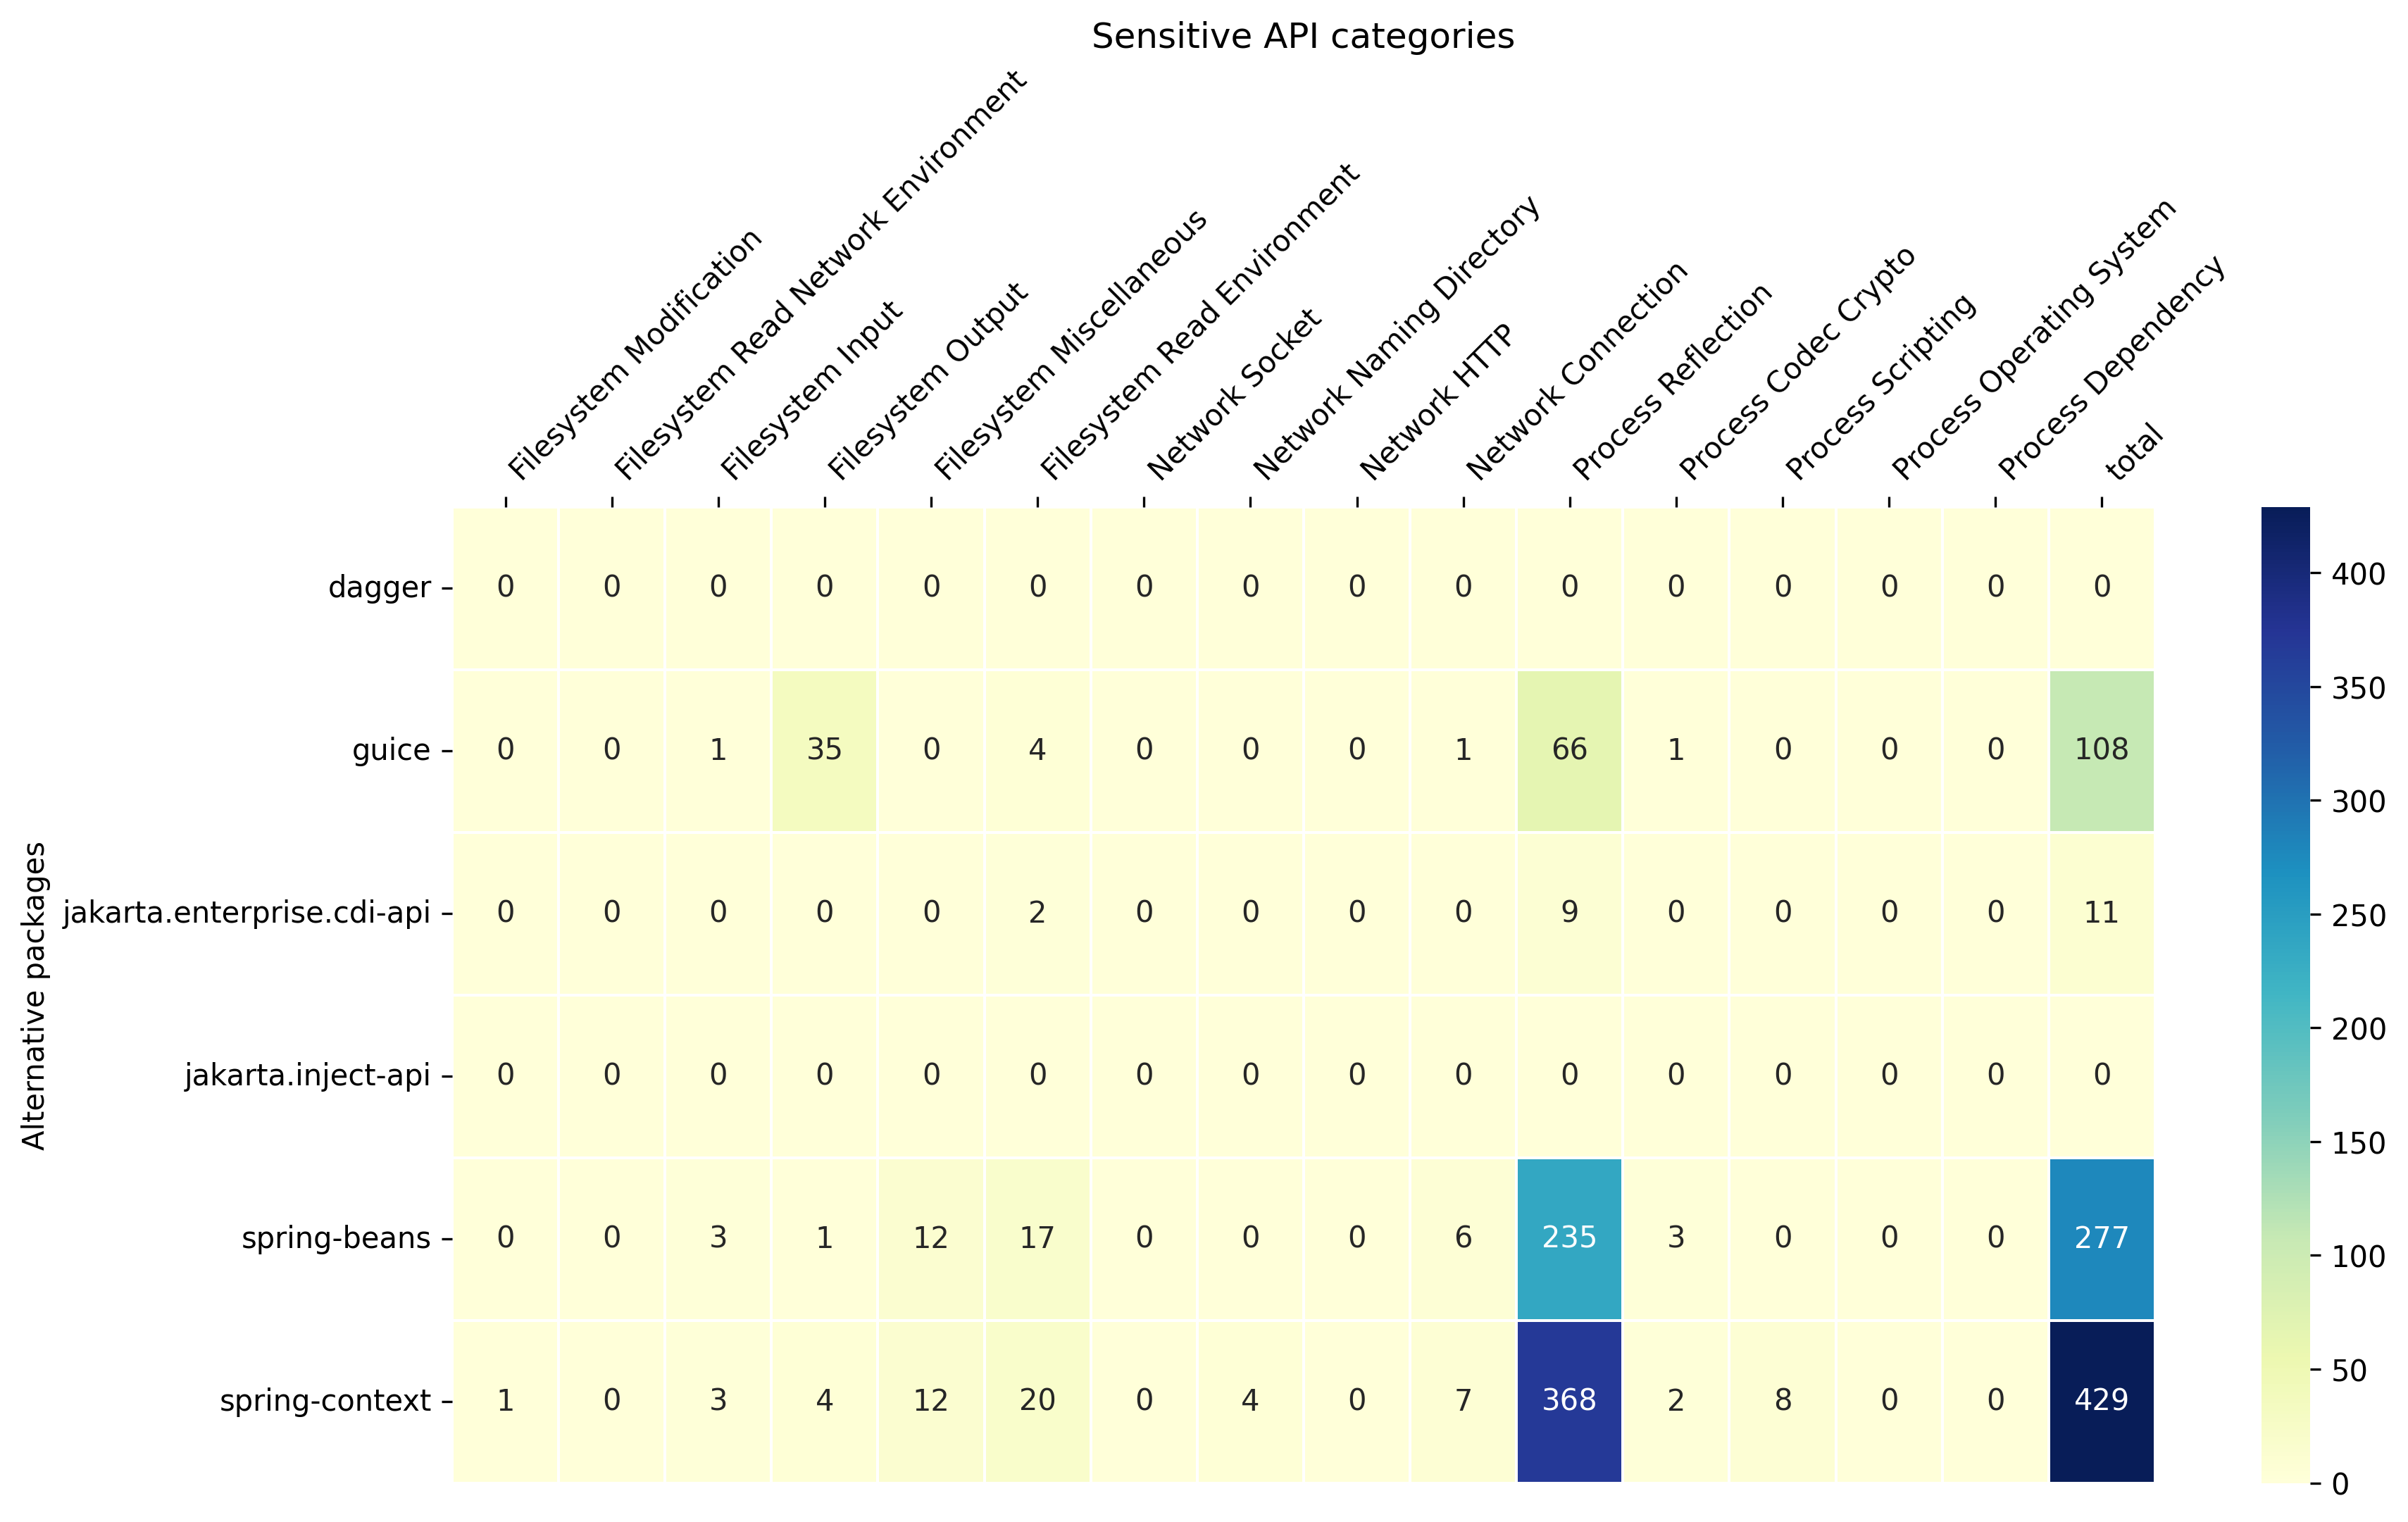}
    \caption{Dependency injection packages' \sensapi usage}
    \label{fig:example_survey}
\end{figure}

\begin{figure}[htbp]
    \centering
    \includegraphics[width=0.7\columnwidth]{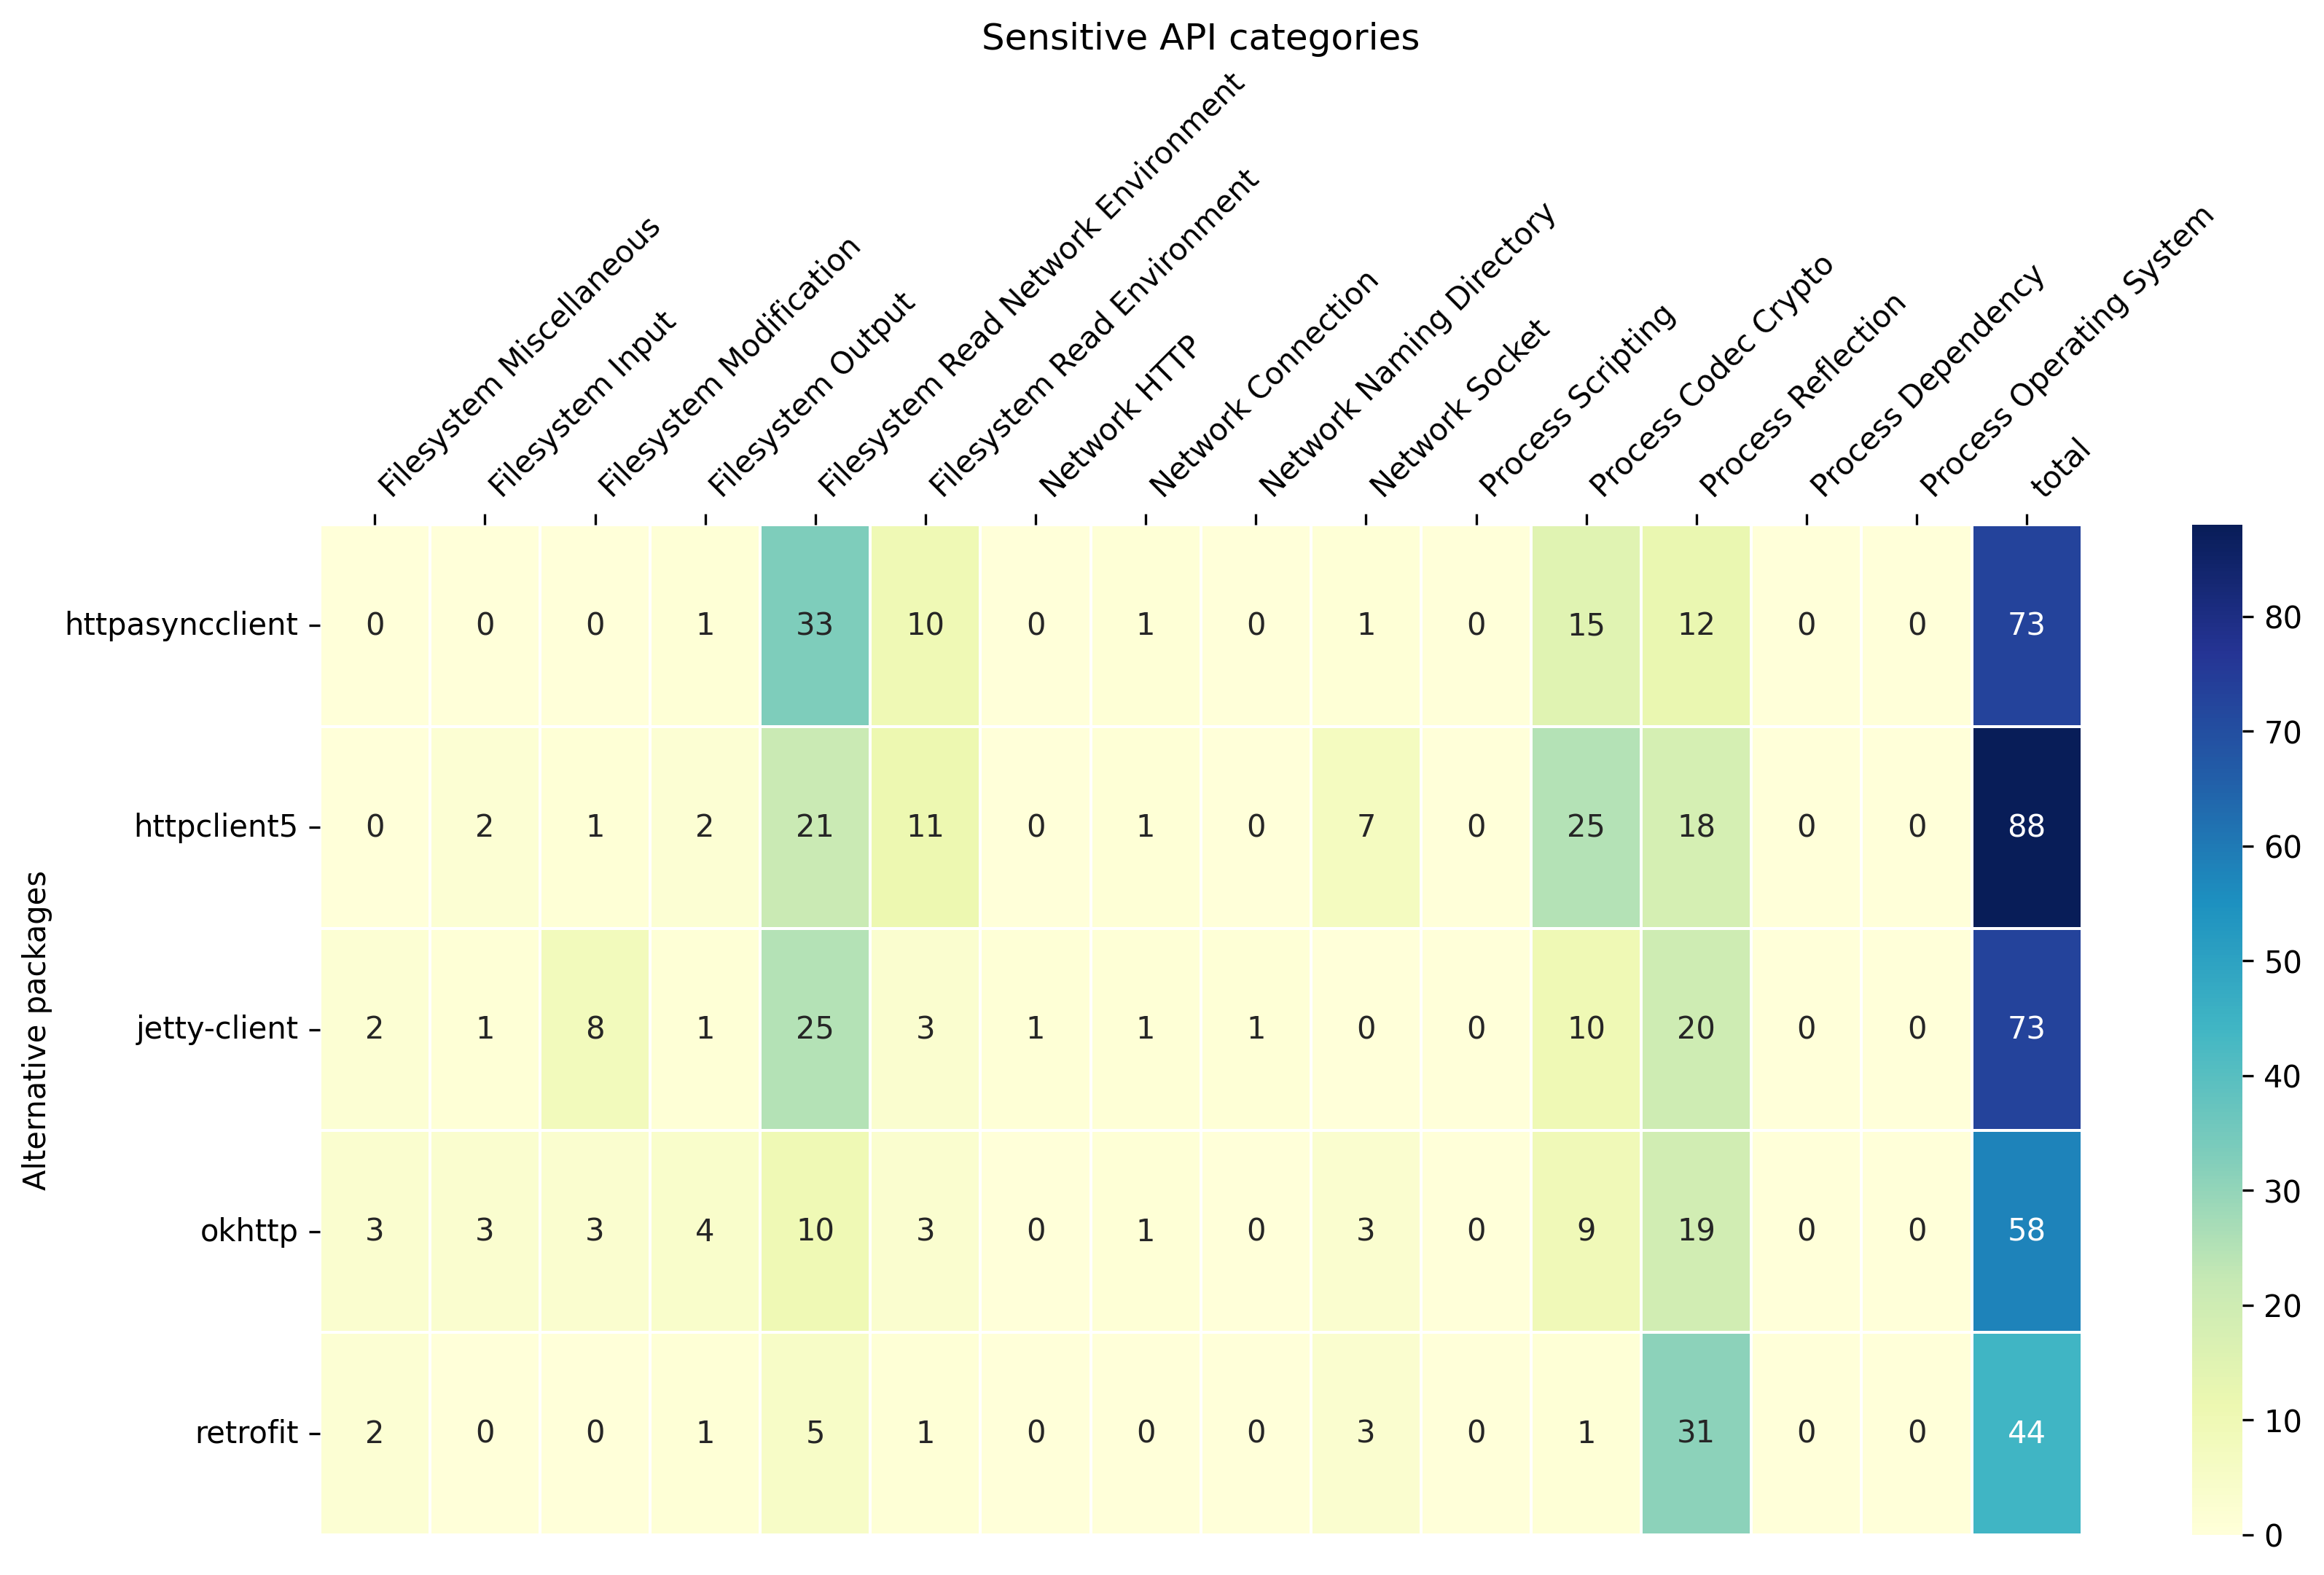}
    \caption{HTTP client packages' \sensapi usage}
    \label{fig:example_survey}
\end{figure}

\begin{figure}[htbp]
    \centering
    \includegraphics[width=0.7\columnwidth]{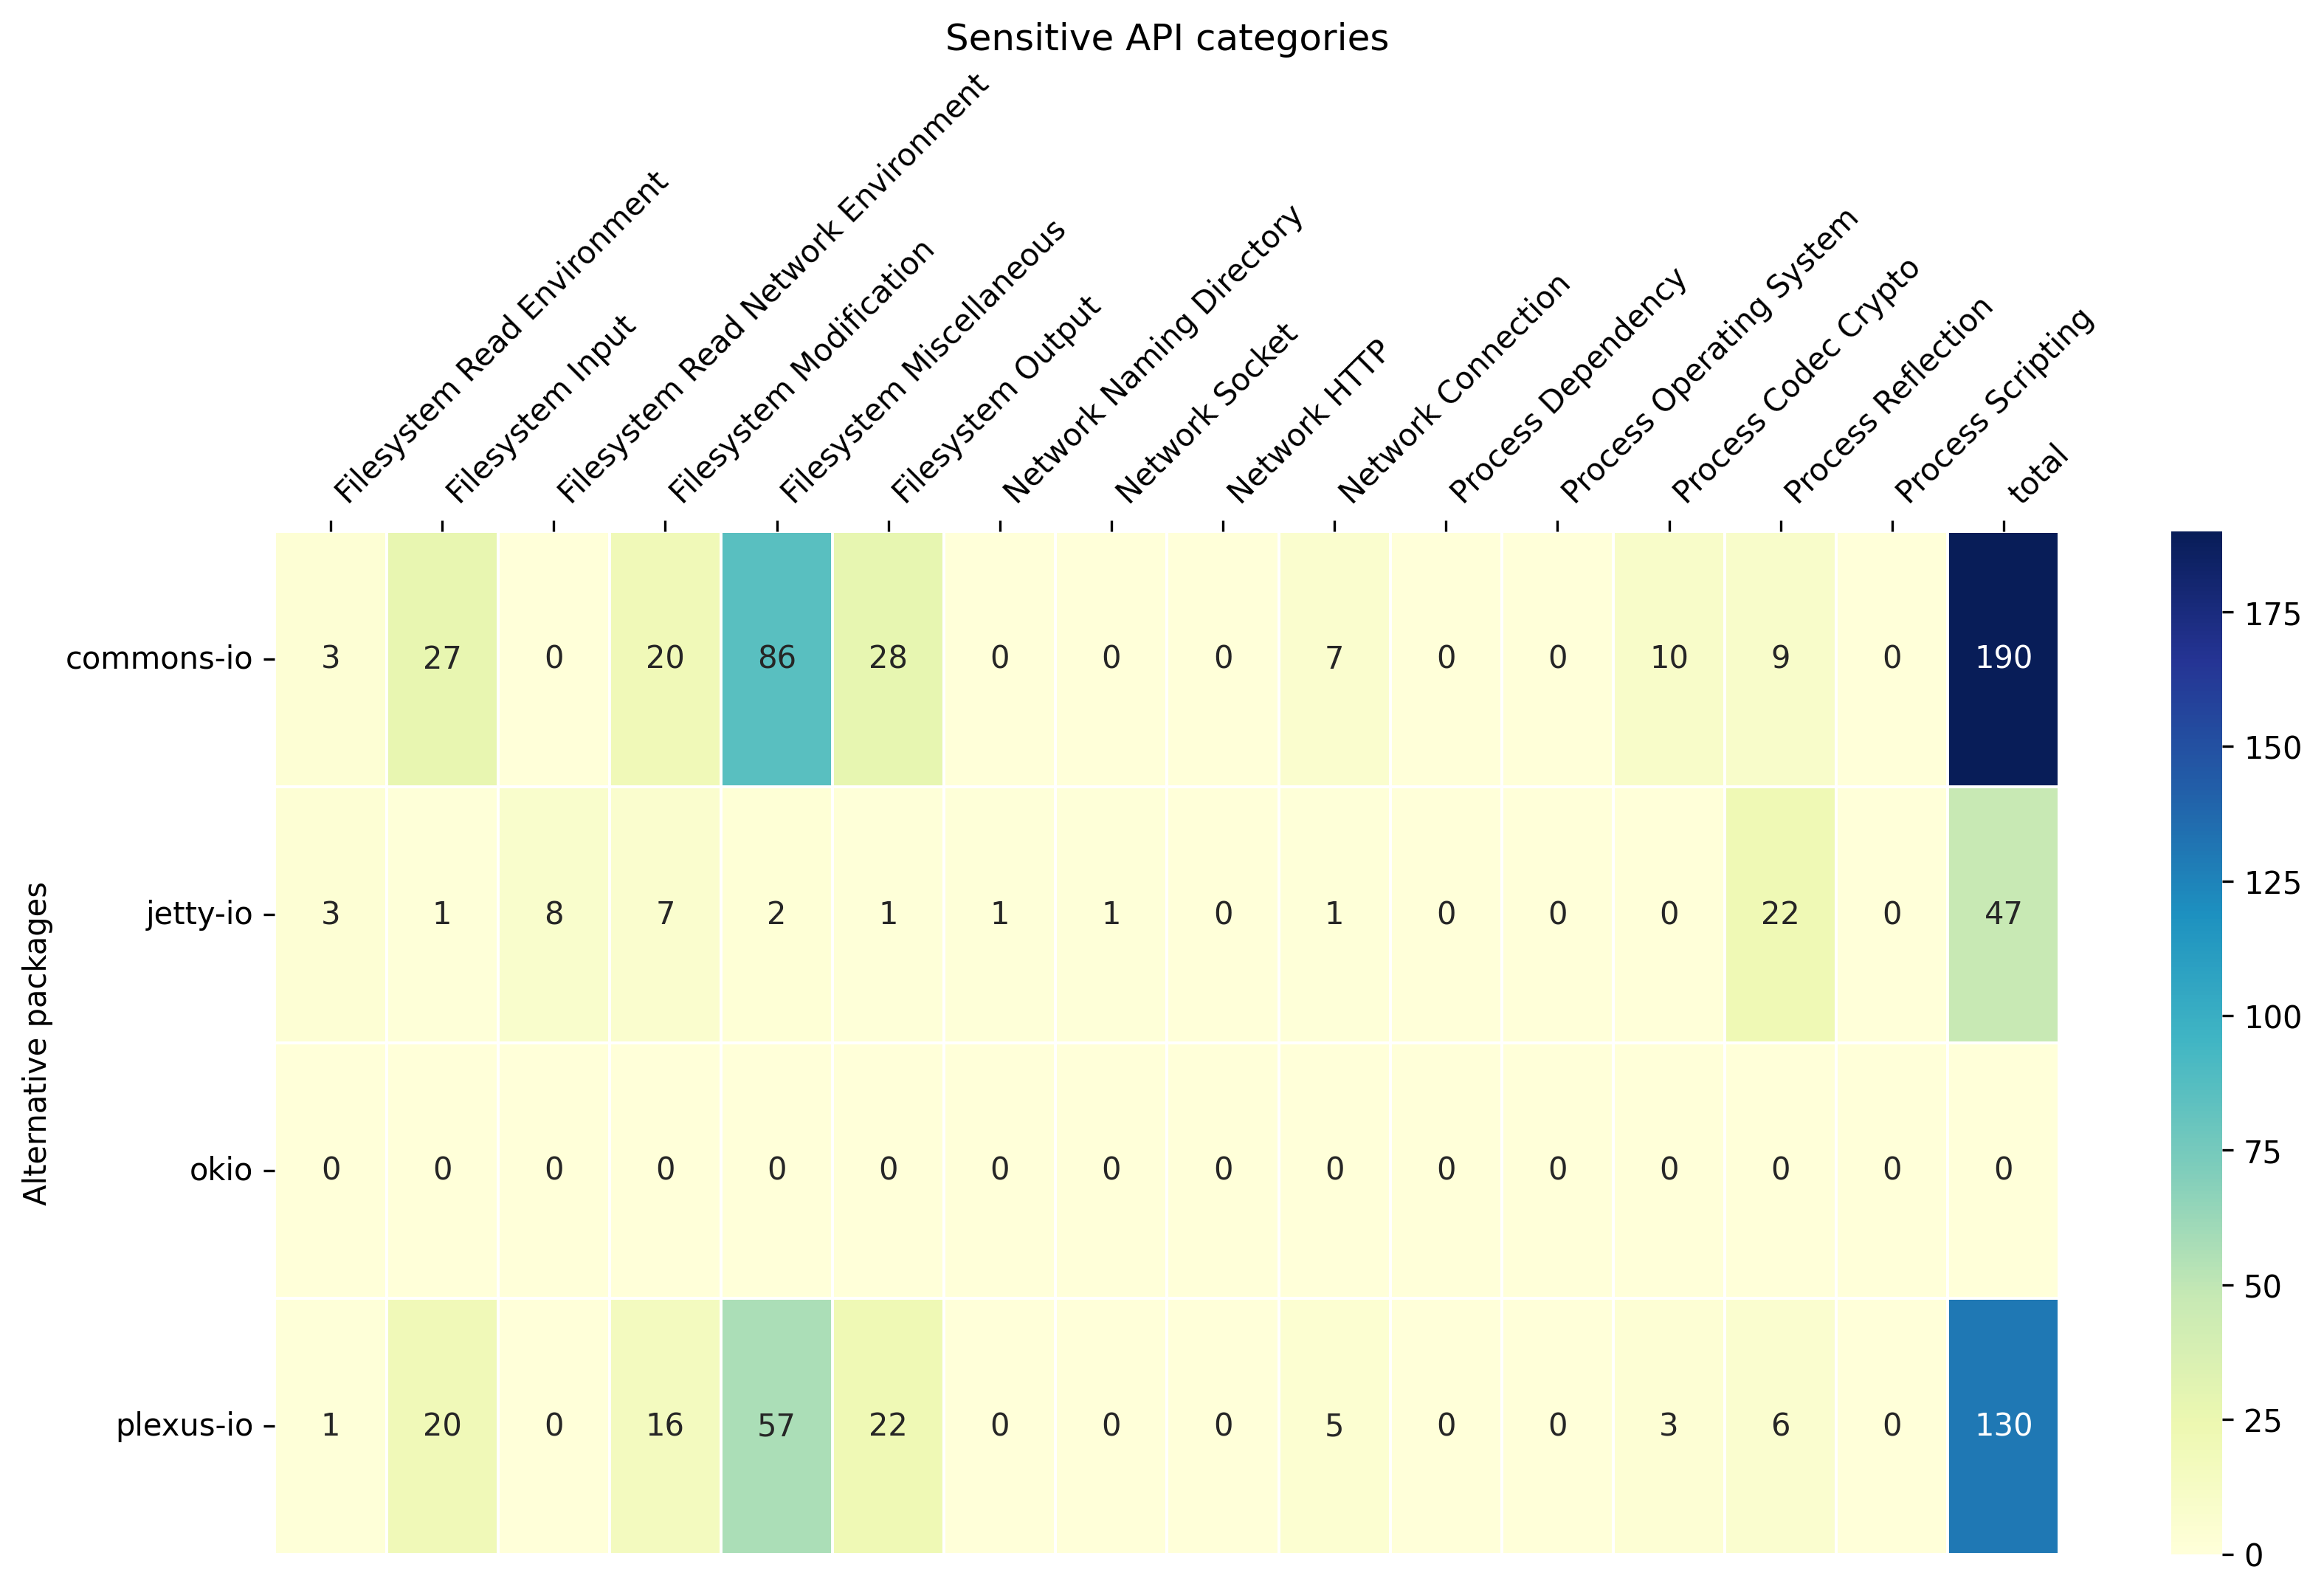}
    \caption{I/O utility packages' \sensapi usage}
    \label{fig:example_survey}
\end{figure}

\begin{figure}[htbp]
    \centering
    \includegraphics[width=0.7\columnwidth]{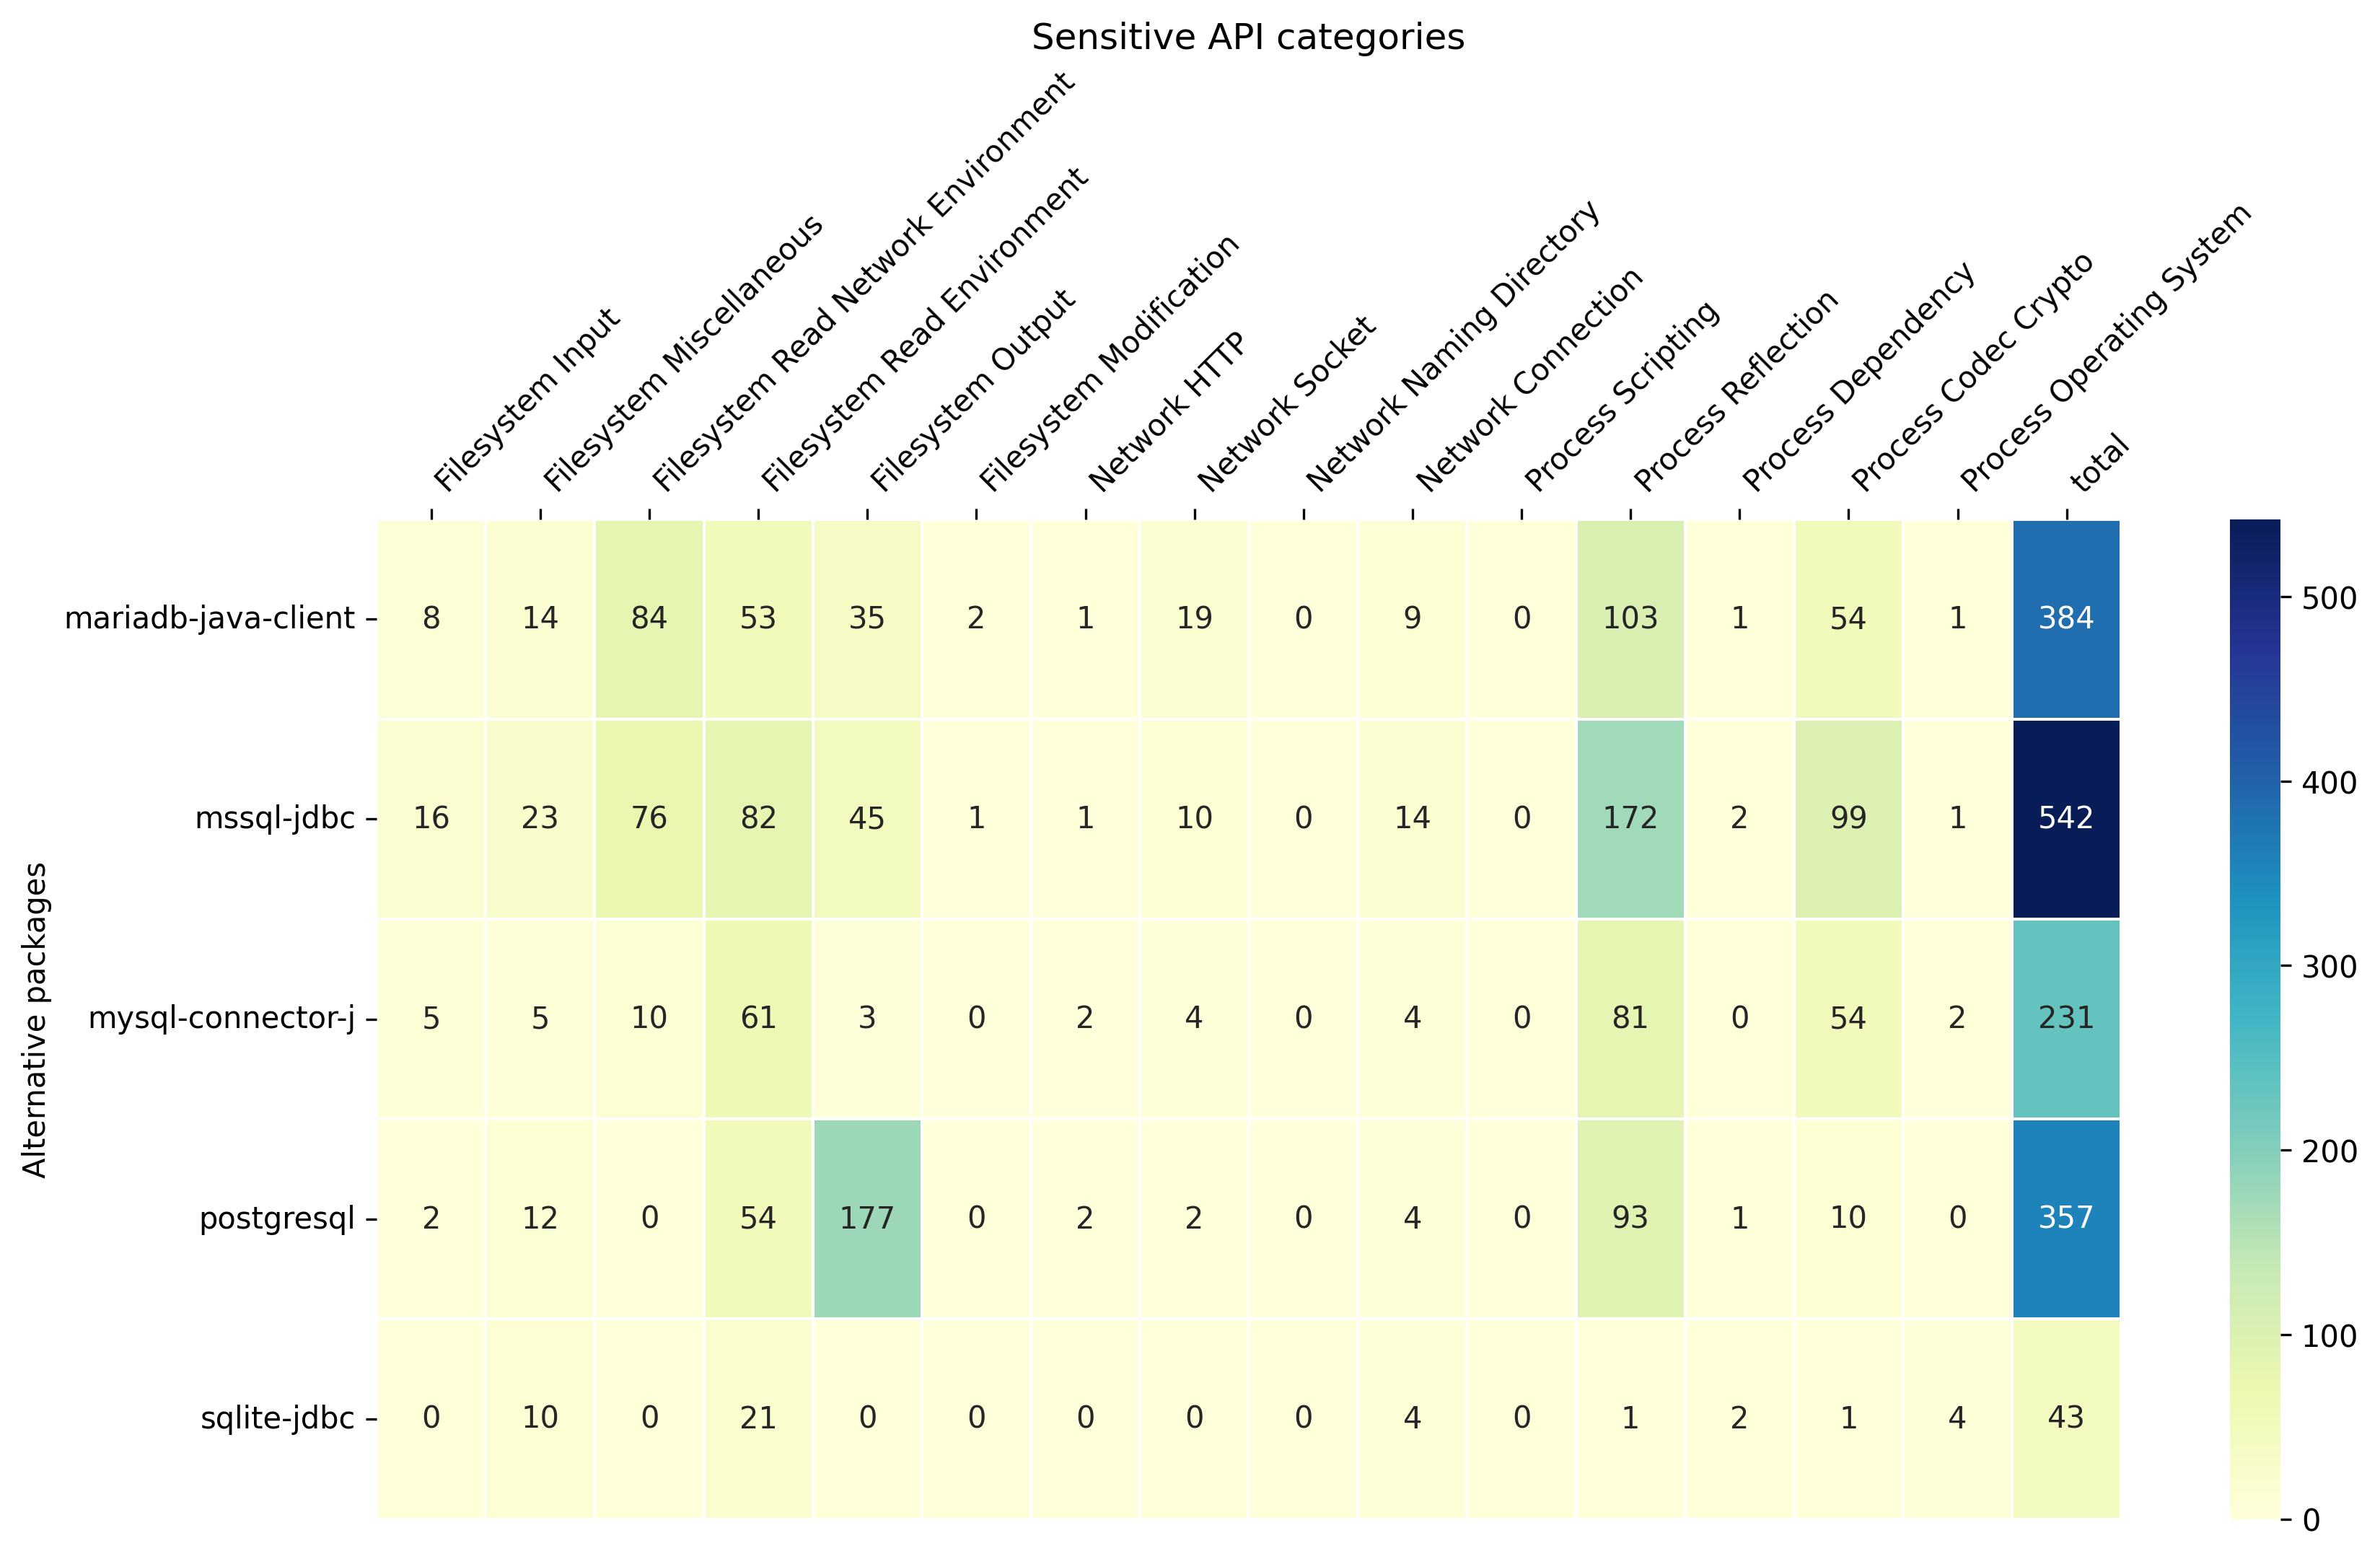}
    \caption{JDBC driver packages' \sensapi usage}
    \label{fig:example_survey}
\end{figure}

\begin{figure}[htbp]
    \centering
    \includegraphics[width=0.7\columnwidth]{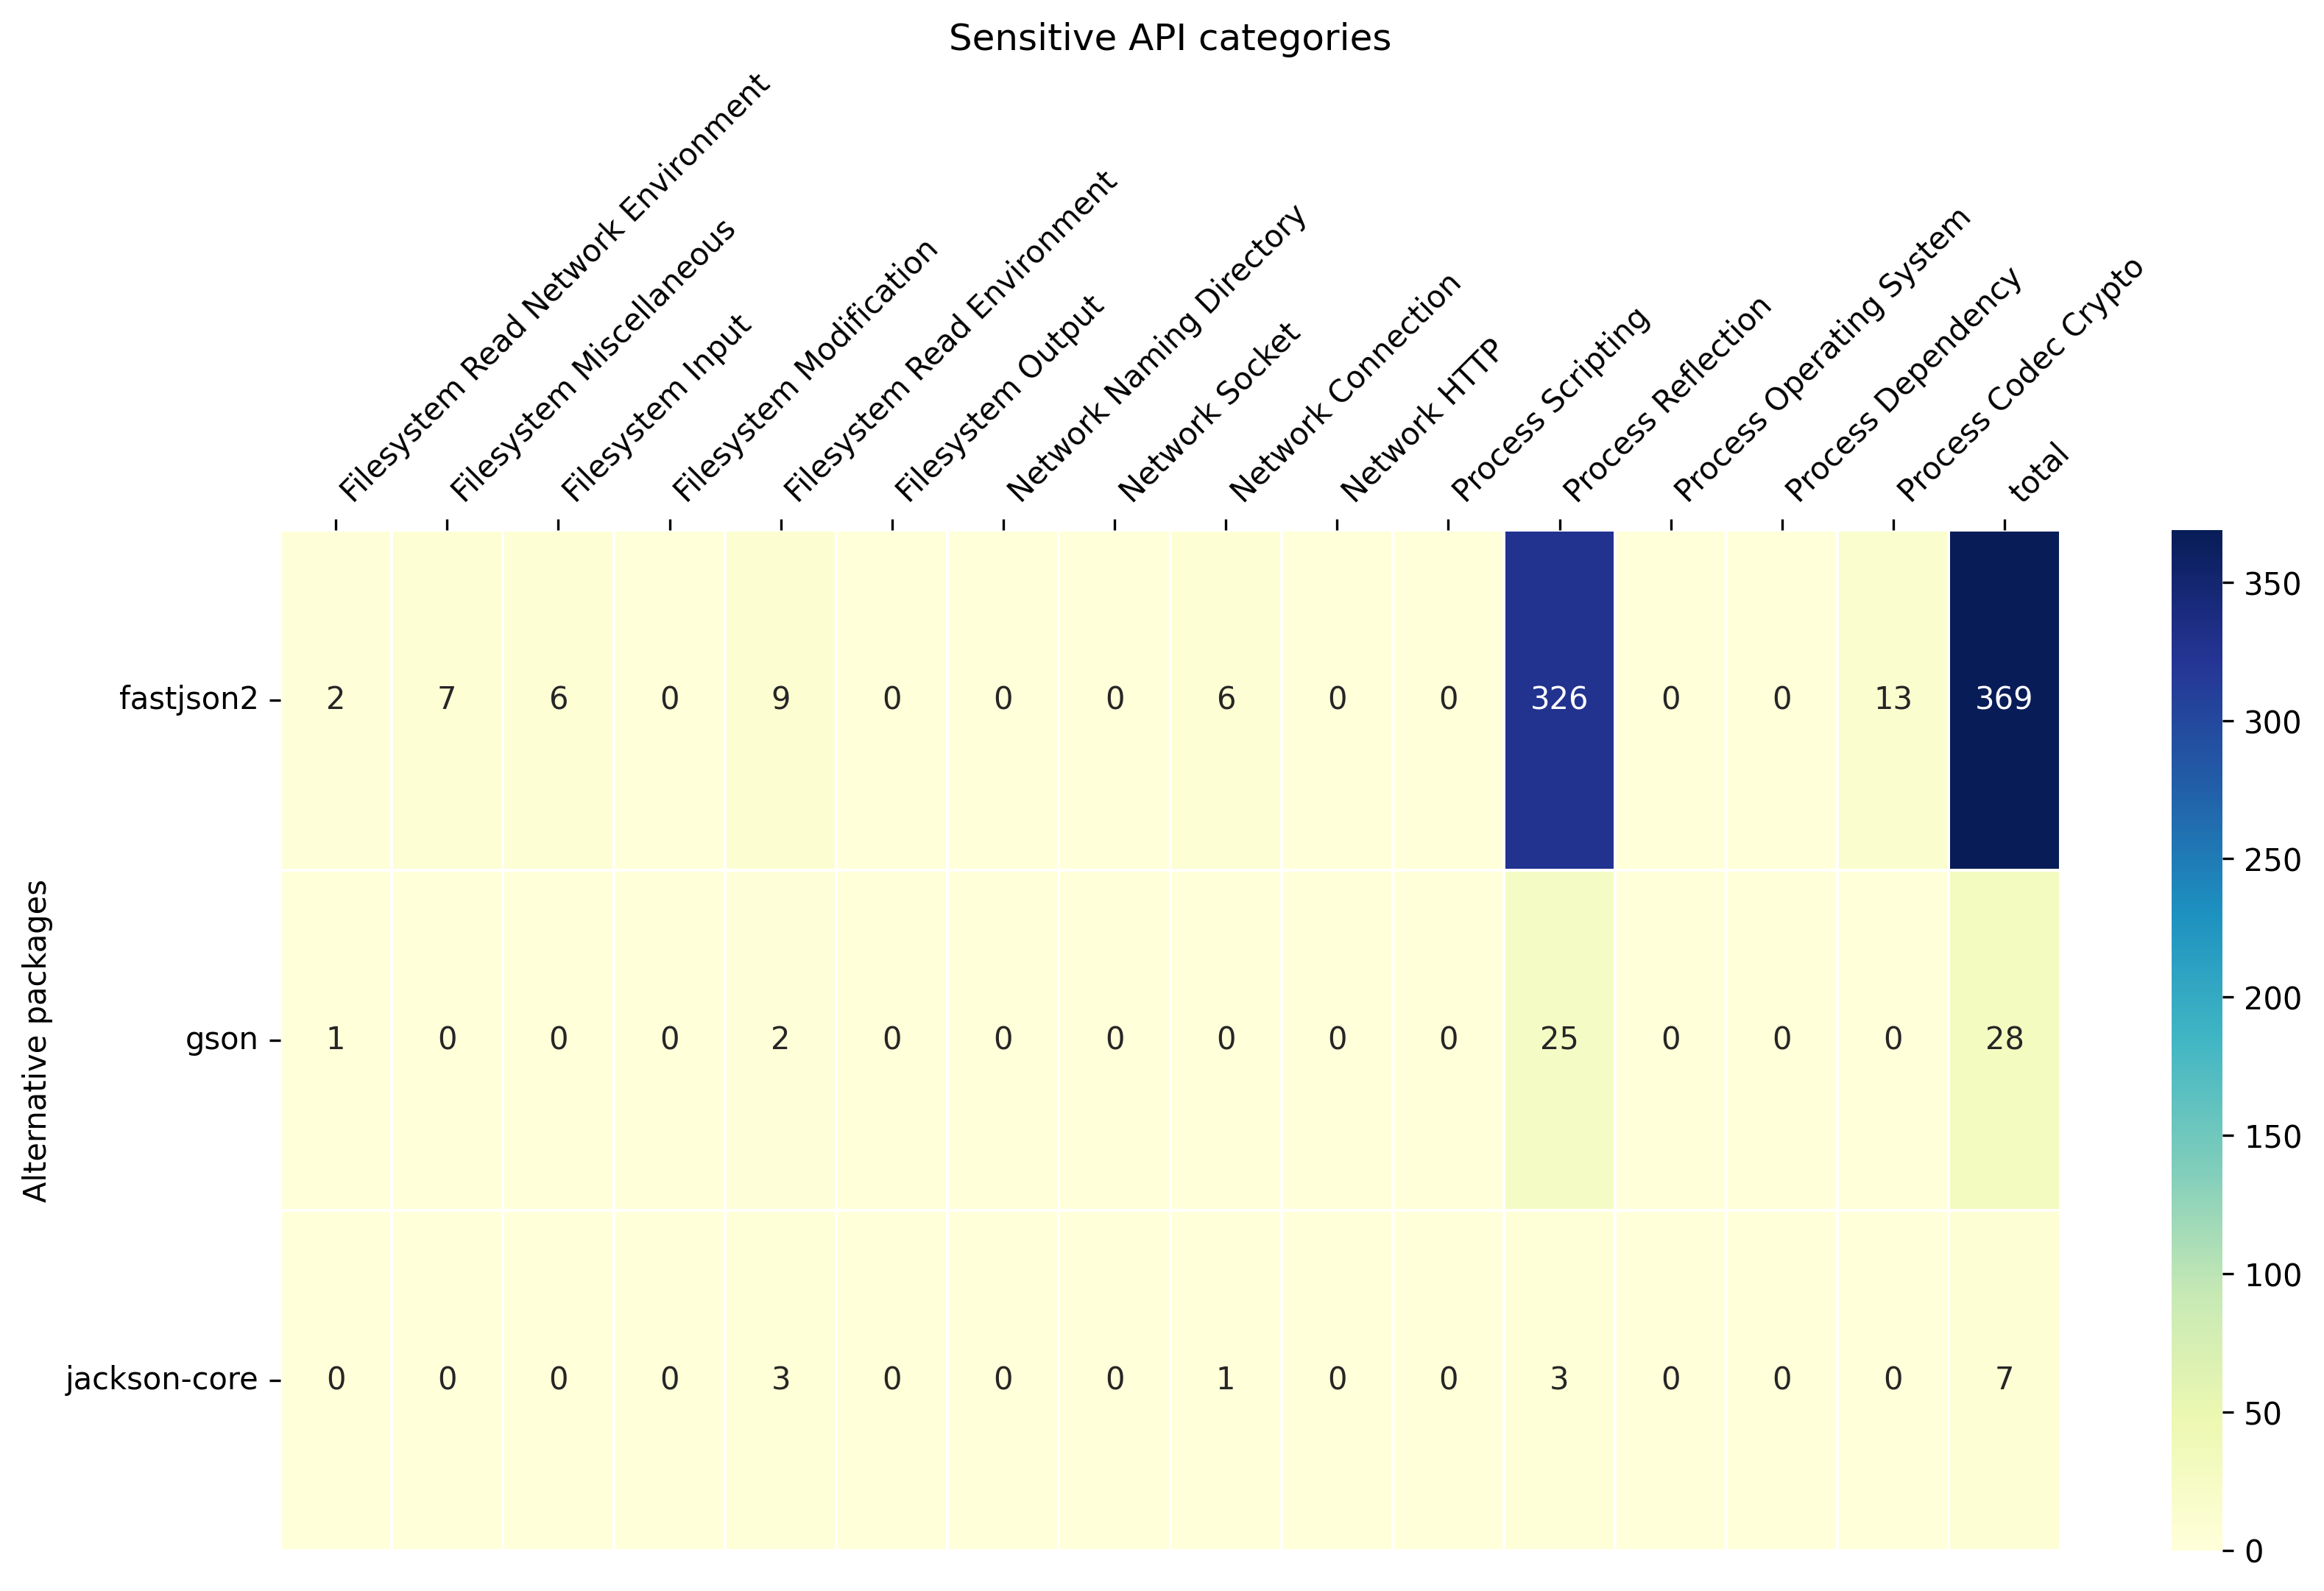}
    \caption{JSON library packages' \sensapi usage}
    \label{fig:example_survey}
\end{figure}

\begin{figure}[htbp]
    \centering
    \includegraphics[width=0.7\columnwidth]{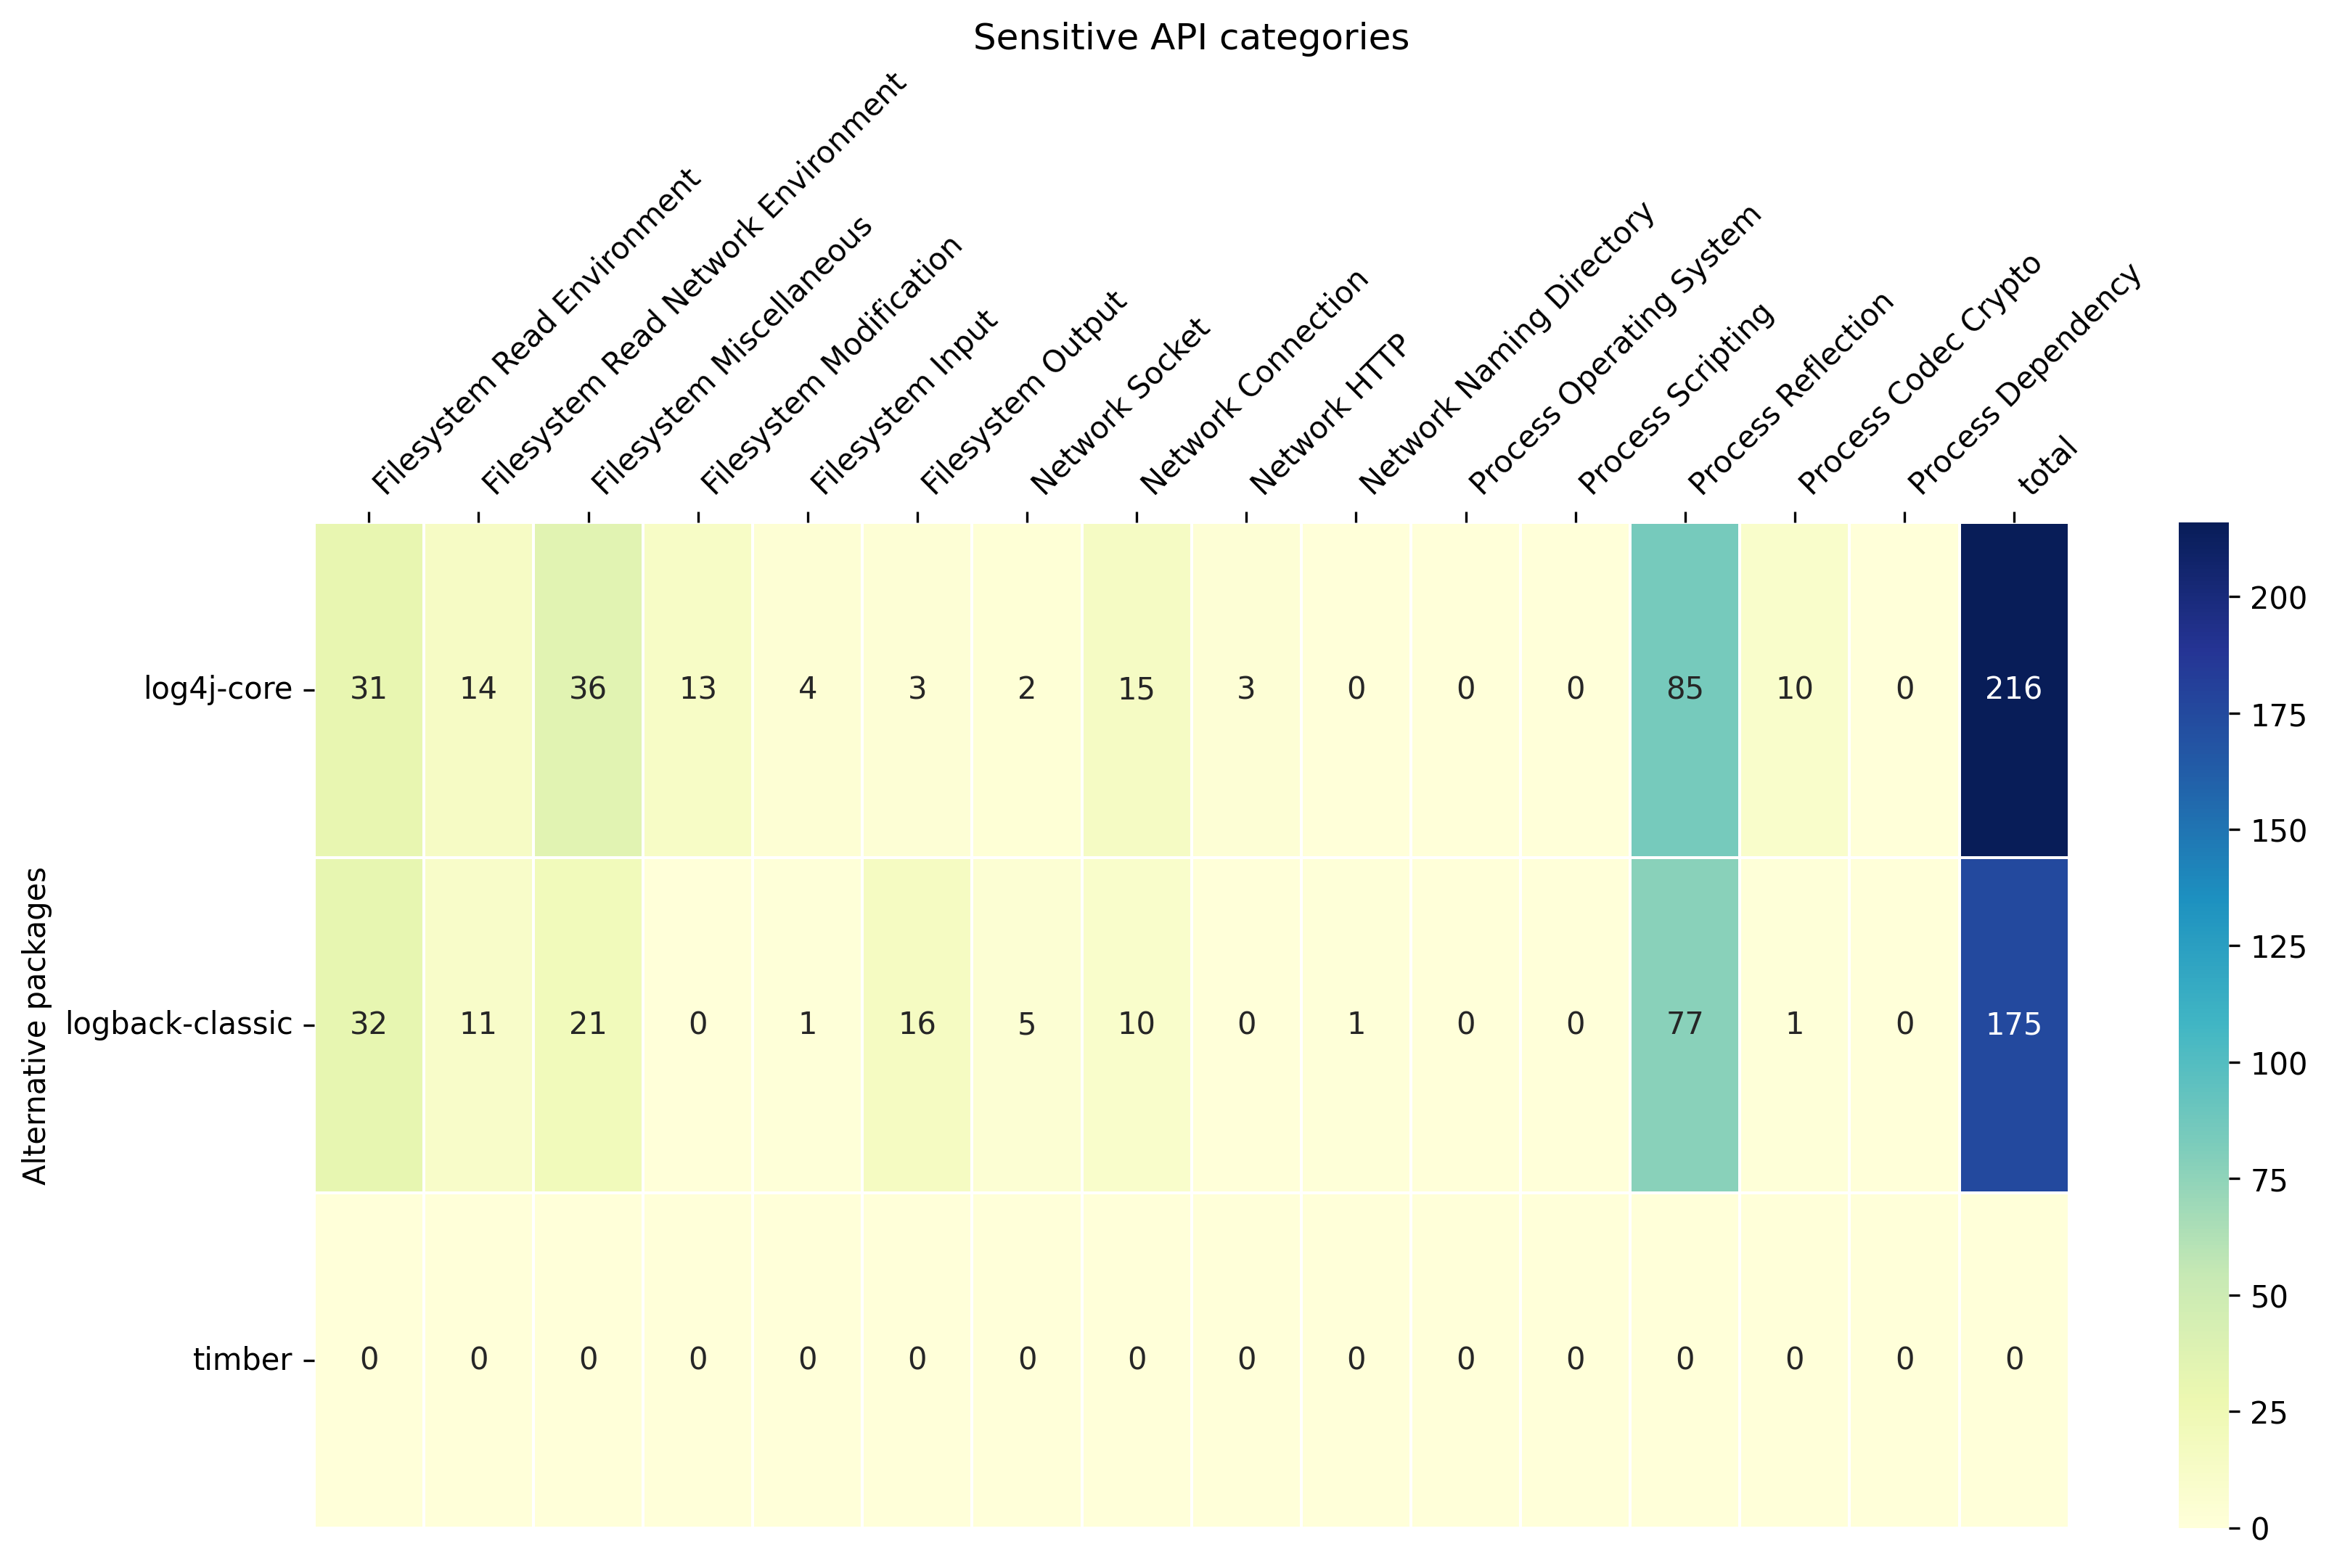}
    \caption{Logging packages' \sensapi usage}
    \label{fig:example_survey}
\end{figure}

\begin{figure}[htbp]
    \centering
    \includegraphics[width=0.7\columnwidth]{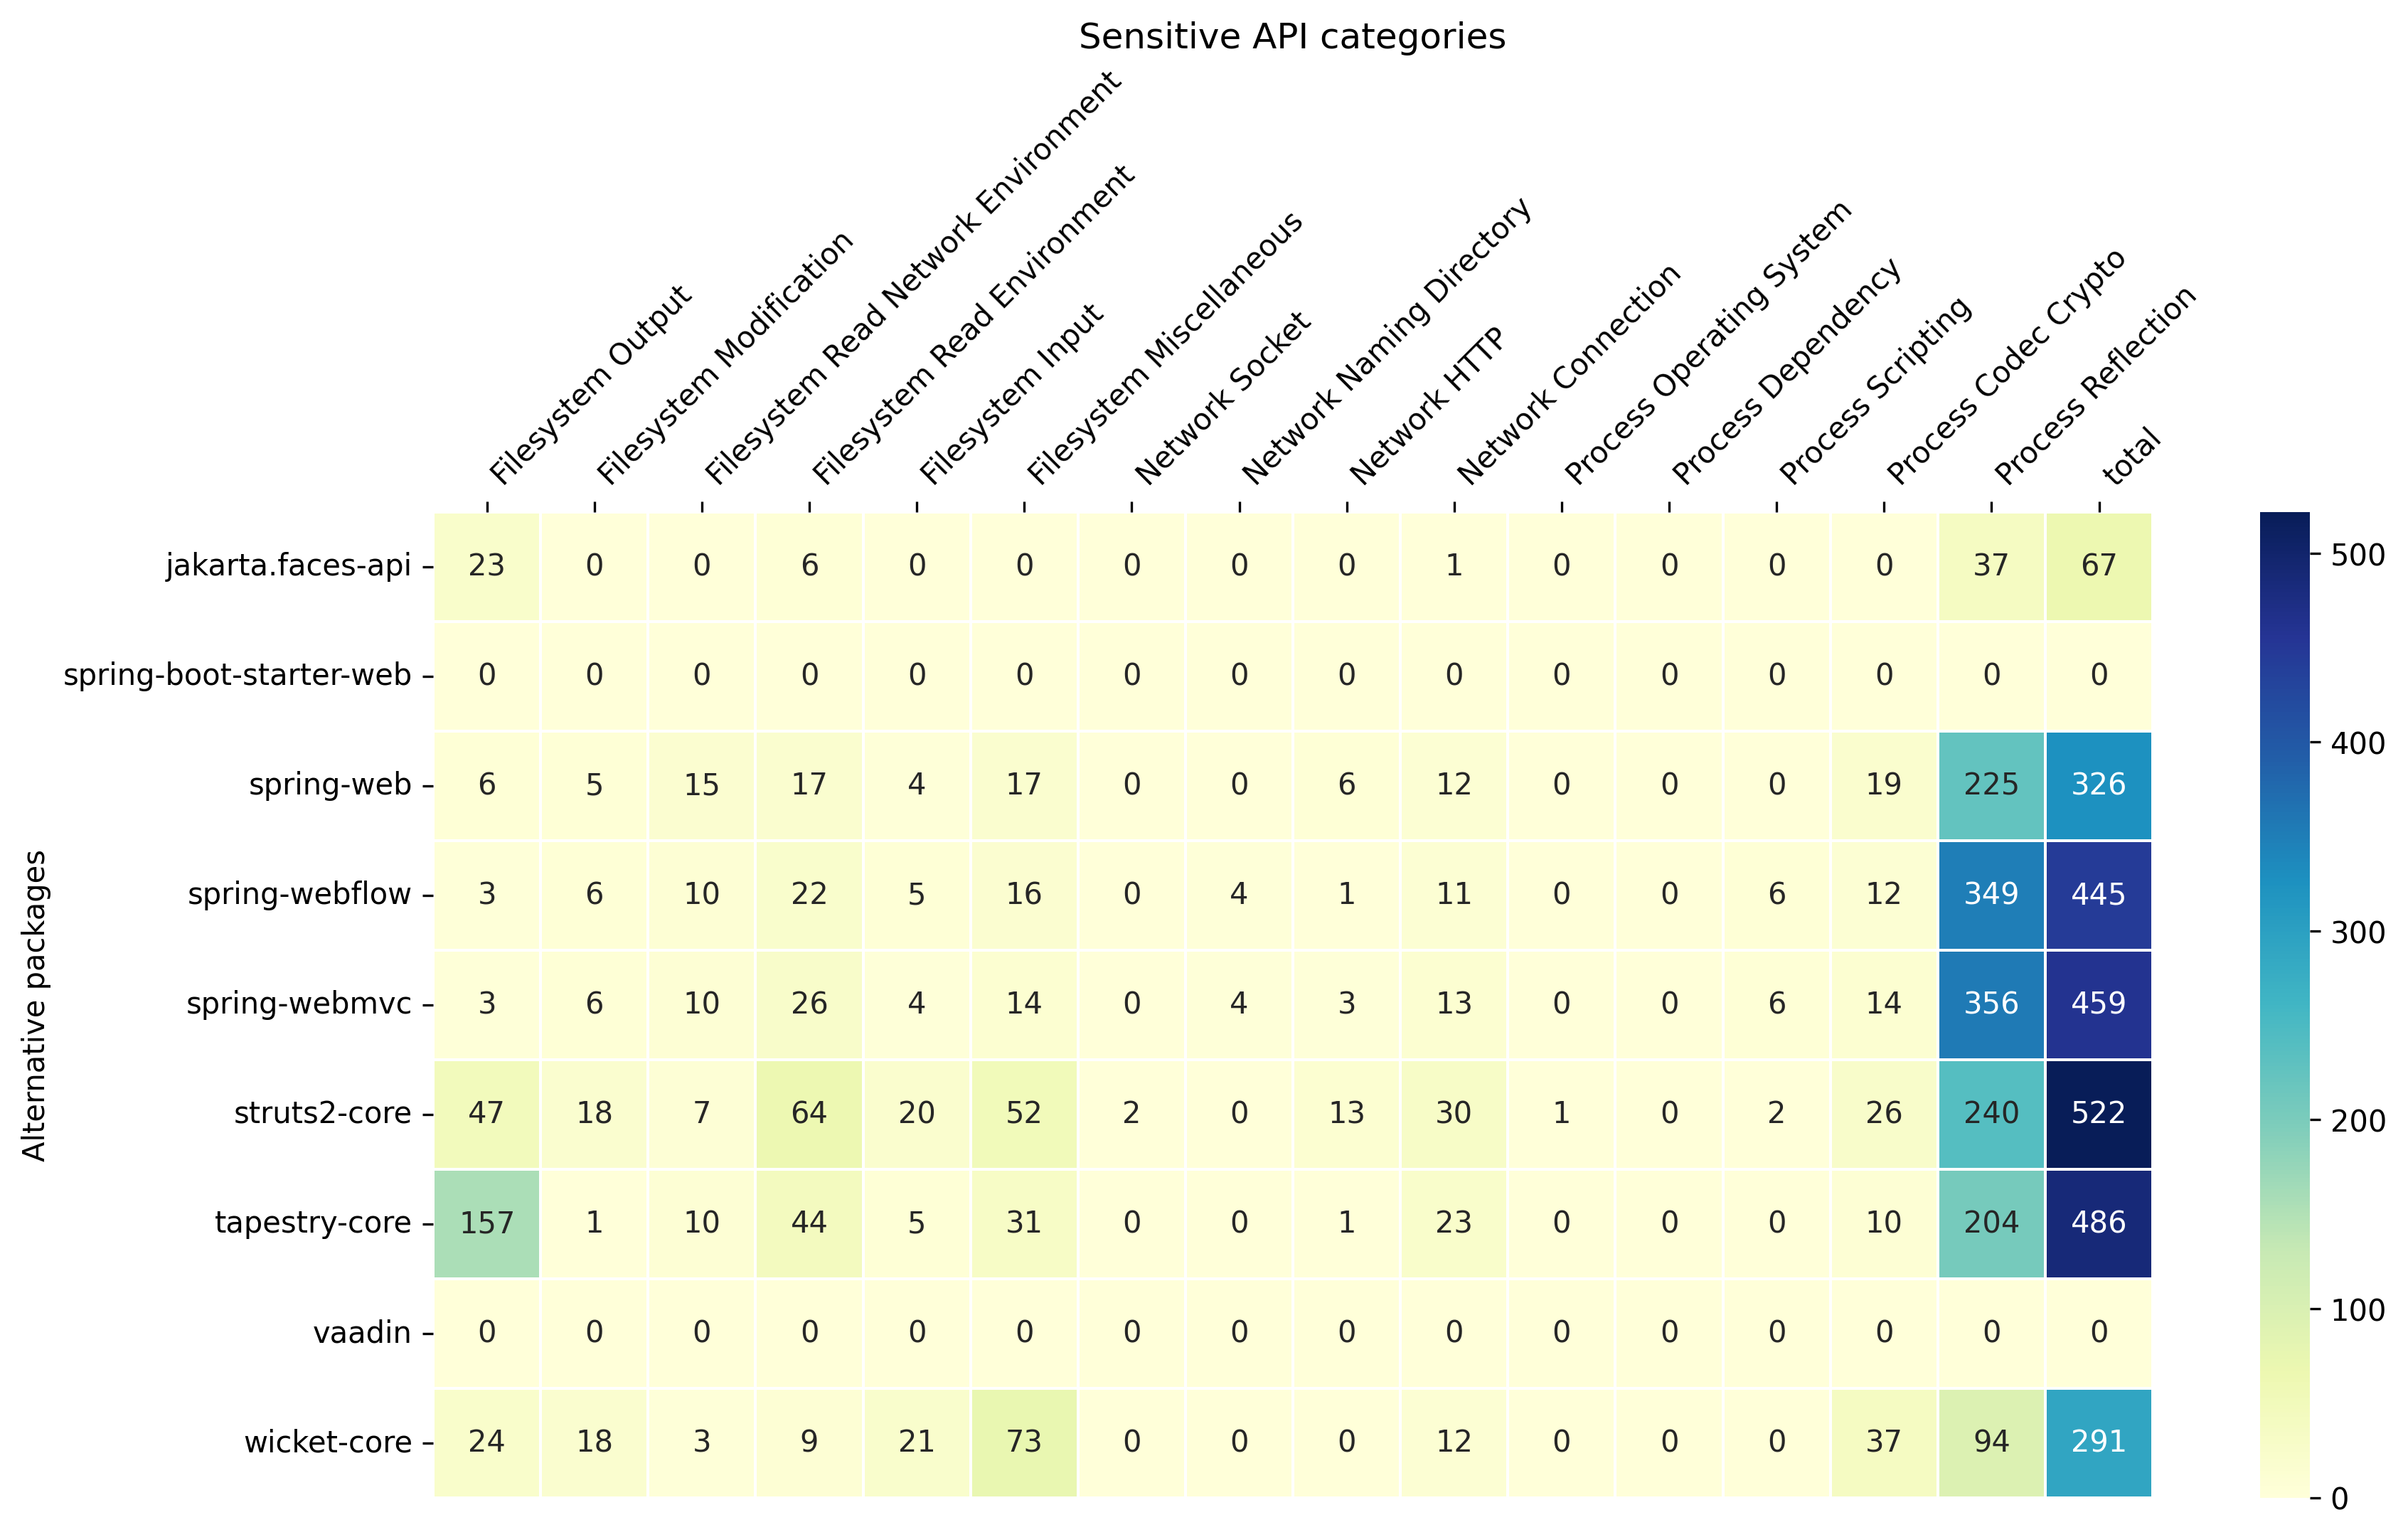}
    \caption{Web framework packages' \sensapi usage}
    \label{fig:example_survey}
\end{figure}

\begin{figure}[htbp]
    \centering
    \includegraphics[width=0.7\columnwidth]{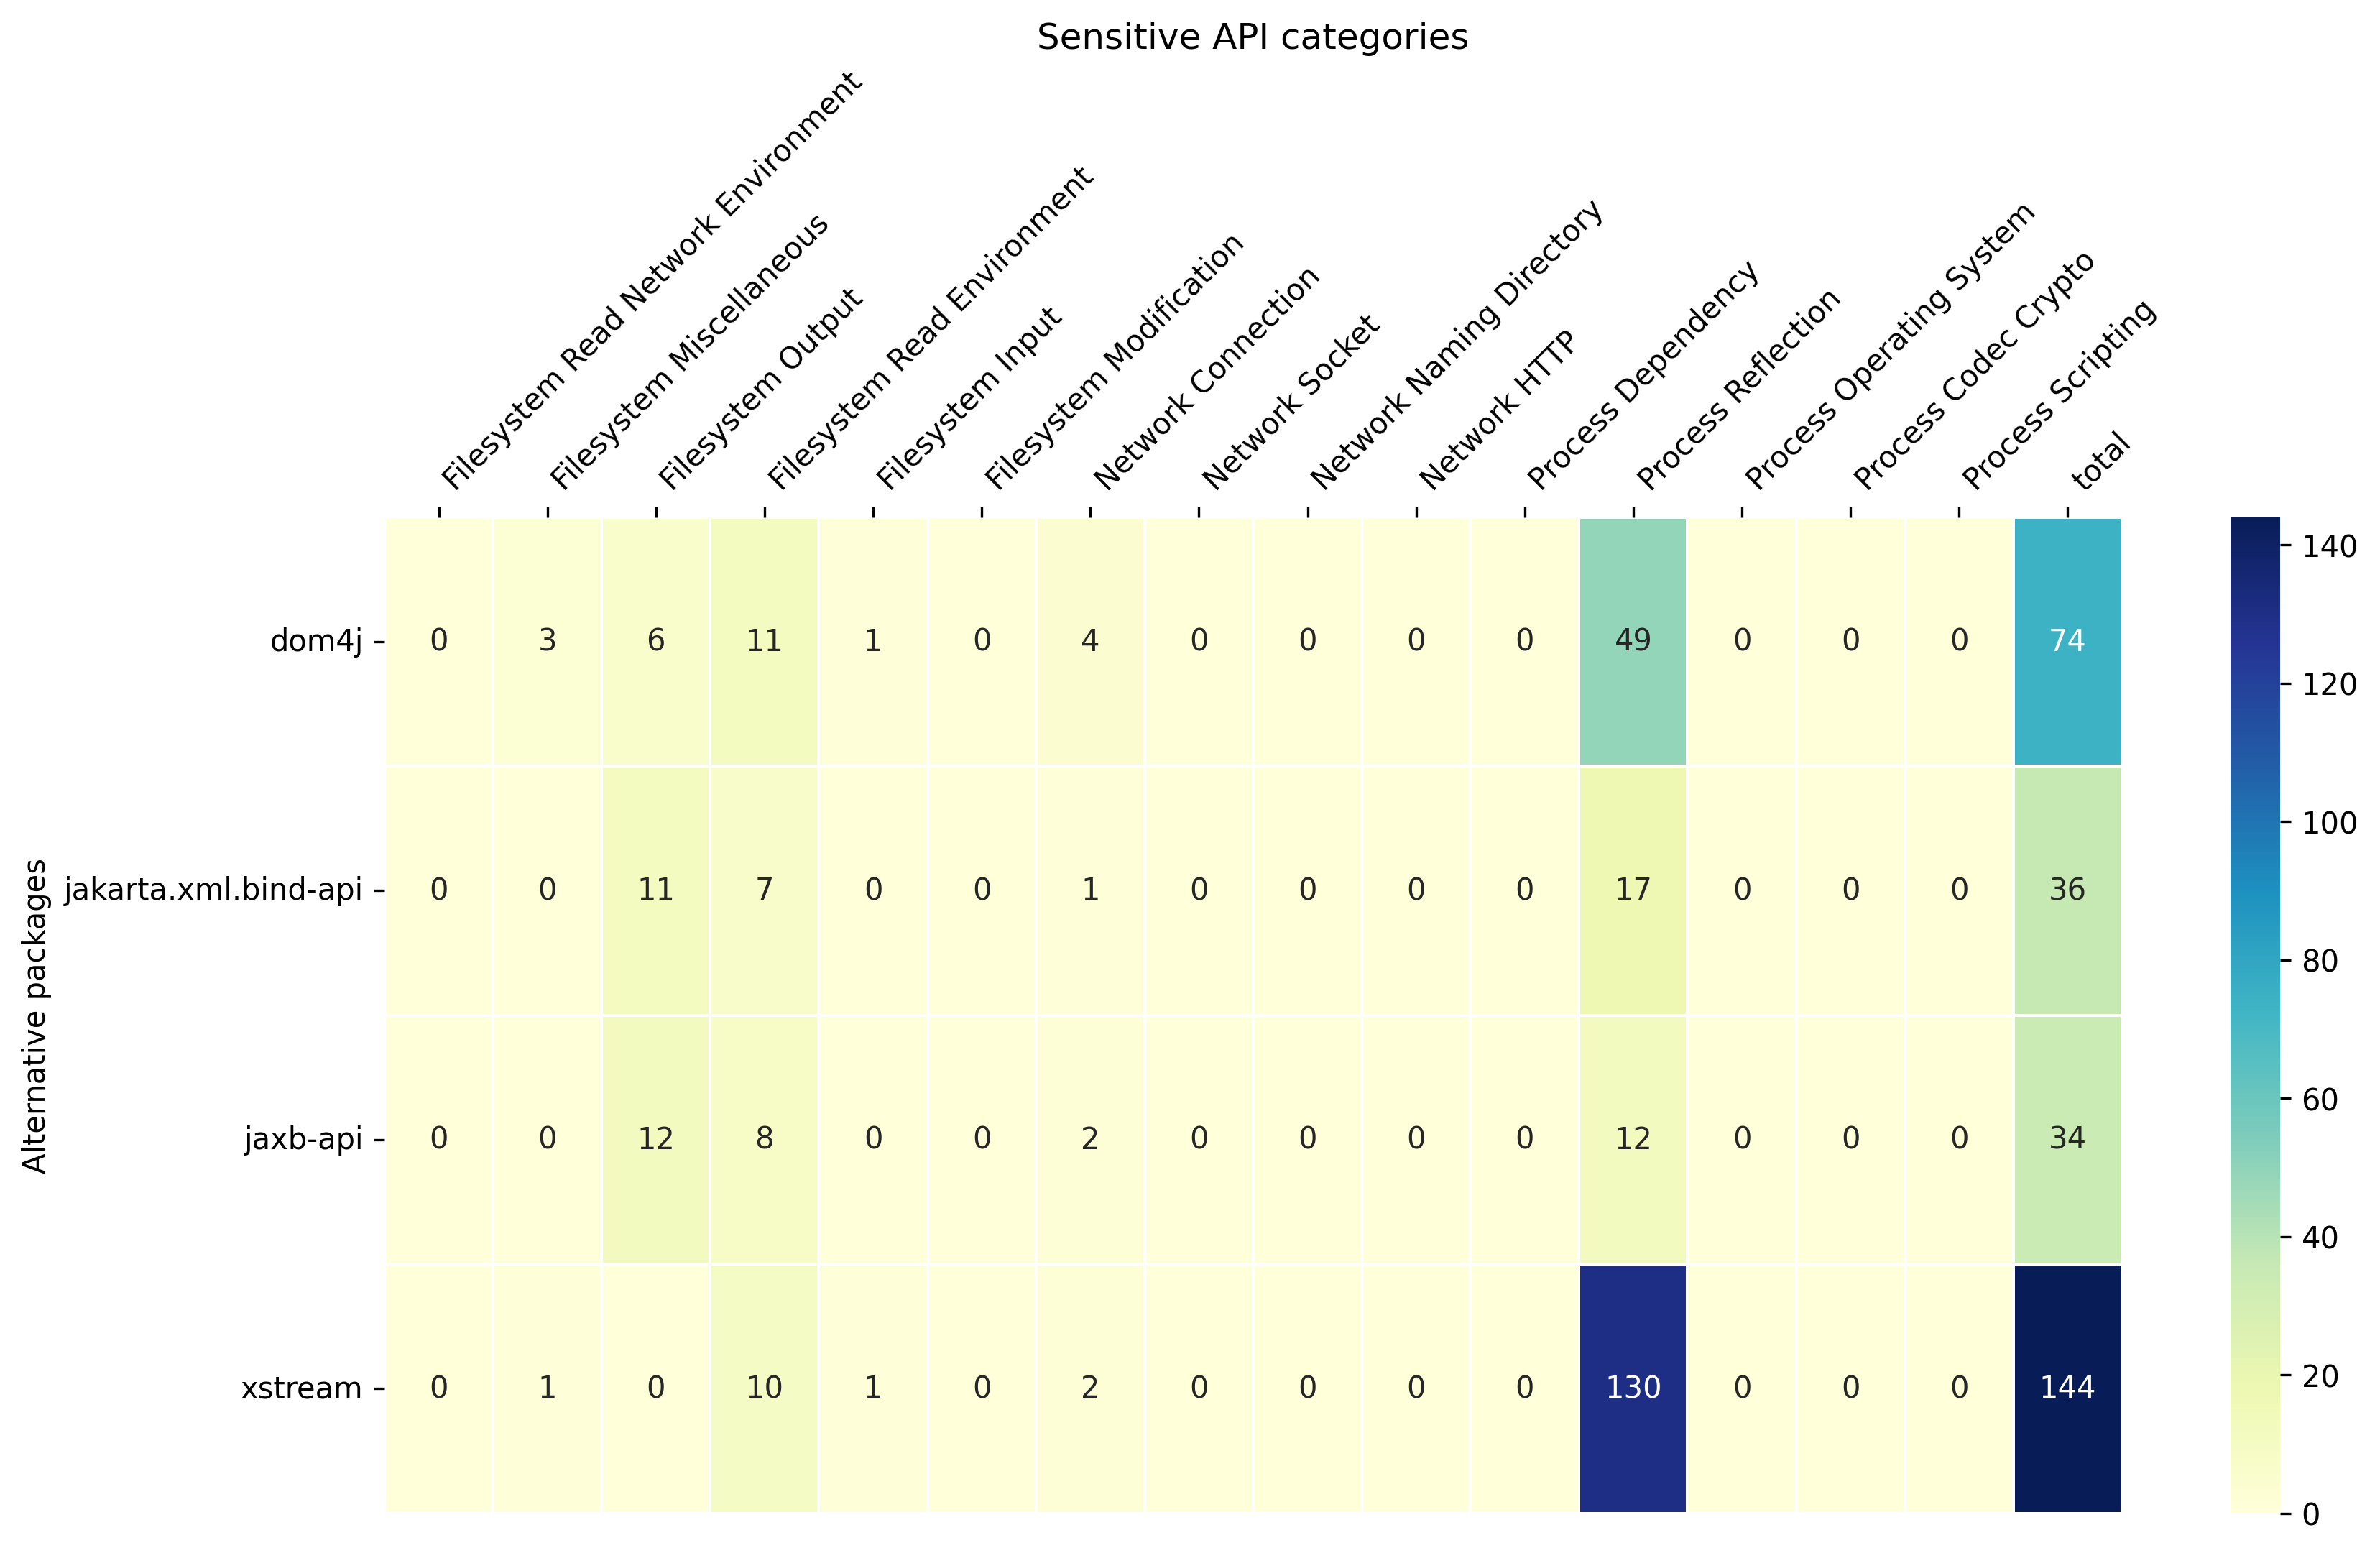}
    \caption{XML parser packages' \sensapi usage}
    \label{fig:example_survey}
\end{figure}

\end{document}
